# Supplementary material for: Discovering Spatial Patterns of Readmission Risk Using a Bayesian Competing Risks Model with Spatially Varying Coefficients
Source: arXiv:2511.20616 ancillary file (2025-11-25)
Supplement: Supplementary file 1 [file Supplement.pdf]

# Supplementary Material of the Manuscript: "Discovering Spatial Patterns of Readmission Risk Using a Bayesian Competing Risk Model with Spatially Varying Coefficients"

Yueming Shen [1,2], Christian A. Pean [3], David B. Dunson [1], and Samuel I. Berchuck [1,2,4]

[1]Department of Statistical Science, Duke University

[2]Duke AI Health, Duke University

[3] Department of Orthopaedic Surgery, Duke University

[4]Department of Biostatistics and Bioinformatics, Duke University

November 25, 2025

## Introduction

This document provides supplementary material to the paper entitled "Discovering Spatial Patterns of Readmission Risk Using a Bayesian Competing Risk Model with Spatially Varying Coefficients". It is organized into seven sections. Section 1 lists the inclusion and exclusion Current Procedural Terminology (CPT) and International Classification of Diseases (ICD) codes used to define the patient cohort. Section 2 summarizes cohort demographics. Section 3 describes how insurance types were grouped from the raw Electronic Health Records (EHR) data. Section 4 presents a proof of the kriging distribution under the Hilbert space Gaussian process (HSGP) approximation. Sections 5 and 6 provide additional results from the simulation study and the EHR application, respectively. Section 7 reports the sensitivity analysis results.

# 1 Inclusion and exclusion criteria

In this section, we provide the CPT and ICD codes used for creating the patient cohort for our EHR data.

## 1.1 CPT codes

We included patients associated with the following CPT codes:

23515, 23585, 23615, 23616, 23630, 24515, 24516, 24538, 24545, 24546, 24575, 24579, 24586, 24587, 24615, 24635, 24665, 24666, 24685, 25515, 25525, 25526, 25545, 25574, 25575, 25607, 25608, 25609.

We excluded patients associated with the following CPT codes:

25900, 25920, 26952, 24800, 24900, 27215, 27217, 27218, 27226, 27227, 27228, 27125, 27187, 27235, 27236, 27244, 27245, 27248, 27253, 27254, 27258, 27269, 27506, 27507, 27509, 27511, 27513, 27514, 27519, 27524, 27535, 27536, 27590, 27591, 27592, 27756, 27758, 27759, 27766, 27769, 27784, 27792, 27814, 27822, 27823, 27826, 27827, 27828, 27880, 27881, 27882, 27420, 28445, 28800, 28805.

## 1.2 ICD codes

We used ICD codes to identify a broad orthopaedic patient population with fragility fracture, osteoarthritis, or osteoporosis. Only patients in this broad population were further considered for the study.

### 1.2.1 Fragility fracture ICD codes

ICD-9 Codes:

820.00, 820.01, 820.02, 820.03, 820.09, 820.10, 820.11, 820.12, 820.13, 820.19, 820.20,

820.21, 820.22, 820.30, 820.31, 820.32, 820.8, 820.9, 733.14, 813.40, 813.47, 733.12, 812.00, 812.09, 812.20, 812.21, 812.40, 812.49, 733.11, 733.10, 733.16, 733.19, 805.00, 805.01, 805.02, 805.03,805.04, 805.05, 805.06, 805.07, 805.2, 805.4, 805.8, 806.0, 806.00, 806.09, 806.20, 806.29, 806.4, 806.8, 733.13, 808.0,808.2, 808.41, 808.42, 808.49, 808.8, 733.14, 733.96, 820.01, 820.02, 820.09, 820.10, 820.11, 820.12, 820.13, 820.19, 820.20, 820.21, 820.22, 820.30, 820.31, 820.32, 820.8, 820.9, 808.0

ICD-10 Codes:

M48.40XA, M48.41XA, M48.42XA, M48.43XA, M48.44XA, M48.45XA, M48.46XA, M48.47XA, M48.48XA, M80.00XA, M80.011A, M80.012A, M80.019A, M80.021A, M80.022A, M80.029A, M80.031A, M80.032A, M80.039A, M80.041A, M80.042A, M80.049A, M80.051A, M80.052A, M80.059A, M80.061A, M80.062A, M80.069A, M80.071A, M80.072A, M80.079A, M80.08XA, M80.80XA, M80.811A, M80.812A, M80.819A, M80.821A, M80.822A, M80.829A, M80.831A, M80.832A, M80.839A, M80.841A, M80.842A, M80.849A, M80.851A, M80.852A, M80.859A, M80.861A, M80.862A, M80.869A, M80.871A, M80.872A, M80.879A, M80.88XA, M80.0AXA, M80.8AXA, M84.311A, M84.312A, M84.319A, M84.321A, M84.322A, M84.329A, M84.331A, M84.332A, M84.333A, M84.334A, M84.339A, M84.341A, M84.342A, M84.343A, M84.350A, M84.351A, M84.352A, M84.353A, M84.359A, M84.361A, M84.362A, M84.363A, M84.364A, M84.369A, M84.371A, M84.372A, M84.373A, M84.374A, M84.375A, M84.376A, M84.38XA, M84.750A, M84.751A, M84.752A, M84.753A, M84.754A, M84.755A, M84.756A, M84.757A, M84.759A, M97.01XA, M97.02XA, M97.11XA, M97.12XA, M97.21XA, M97.22XA, M97.31XA, M97.32XA, M97.41XA, M97.42XA, S12.000A, S12.000B, S12.001A, S12.001B, S12.01XA, S12.01XB, S12.02XA, S12.02XB, S12.030A, S12.030B, S12.031A, S12.031B, S12.040A, S12.040B, S12.041A, S12.041B, S12.090A, S12.090B, S12.091A, S12.091B, S12.100A, S12.100B, S12.101A, S12.101B, S12.110A, S12.110B, S12.111A, S12.111B, S12.112A, S12.112B,

S12.120A, S12.120B, S12.121A, S12.121B, S12.130A, S12.130B, S12.131A, S12.131B, S12.14XA, S12.14XB, S12.150A, S12.150B, S12.151A, S12.151B, S12.190A, S12.190B, S12.191A, S12.191B, S12.200A, S12.200B, S12.201A, S12.201B, S12.230A, S12.230B, S12.231A, S12.231B, S12.24XA, S12.24XB, S12.250A, S12.250B, S12.251A, S12.251B, S12.290A, S12.290B, S12.291A, S12.291B, S12.300A, S12.300B, S12.301A, S12.301B, S12.330A, S12.330B, S12.331A, S12.331B, S12.34XA, S12.34XB, S12.350A, S12.350B, S12.351A, S12.351B, S12.390A, S12.390B, S12.391A, S12.391B, S12.400A, S12.400B, S12.401A, S12.401B, S12.430A, S12.430B, S12.431A, S12.431B, S12.44XA, S12.44XB, S12.450A, S12.450B, S12.451A, S12.451B, S12.490A, S12.490B, S12.491A, S12.491B, S12.500A, S12.500B, S12.501A, S12.501B, S12.530A, S12.530B, S12.531A, S12.531B, S12.54XA, S12.54XB, S12.550A, S12.550B, S12.551A, S12.551B, S12.590A, S12.590B, S12.591A, S12.591B, S12.600A, S12.600B, S12.601A, S12.601B, S12.630A, S12.630B, S12.631A, S12.631B, S12.64XA, S12.64XB, S12.650A, S12.650B, S12.651A, S12.651B, S12.690A, S12.690B, S12.691A, S12.691B, S12.8XXA, S12.9XXA, S22.000A, S22.000B, S22.001A, S22.001B, S22.002A, S22.002B, S22.008A, S22.008B, S22.009A, S22.009B, S22.010A, S22.010B, S22.011A, S22.011B, S22.012A, S22.012B, S22.018A, S22.018B, S22.019A, S22.019B, S22.020A, S22.020B, S22.021A, S22.021B, S22.022A, S22.022B, S22.028A, S22.028B, S22.029A, S22.029B, S22.030A, S22.030B, S22.031A, S22.031B, S22.032A, S22.032B, S22.038A, S22.038B, S22.039A, S22.039B, S22.040A, S22.040B, S22.041A, S22.041B, S22.042A, S22.042B, S22.048A, S22.048B, S22.049A, S22.049B, S22.050A, S22.050B, S22.051A, S22.051B, S22.052A, S22.052B, S22.058A, S22.058B, S22.059A, S22.059B, S22.060A, S22.060B, S22.061A, S22.061B, S22.062A, S22.062B, S22.068A, S22.068B, S22.069A, S22.069B, S22.070A, S22.070B, S22.071A, S22.071B, S22.072A, S22.072B, S22.078A, S22.078B, S22.079A, S22.079B, S22.080A, S22.080B, S22.081A, S22.081B, S22.082A, S22.082B, S22.088A, S22.088B, S22.089A, S22.089B, S22.20XA, S22.20XB, S22.21XA, S22.21XB, S22.22XA, S22.22XB, S22.23XA, S22.23XB,

S22.24XA, S22.24XB, S22.31XA, S22.31XB, S22.32XA, S22.32XB, S22.39XA, S22.39XB, S22.41XA, S22.41XB, S22.42XA, S22.42XB, S22.43XA, S22.43XB, S22.49XA, S22.49XB, S22.5XXA, S22.5XXB, S22.9XXA, S22.9XXB, S32.000A, S32.000B, S32.001A, S32.001B, S32.002A, S32.002B, S32.008A, S32.008B, S32.009A, S32.009B, S32.010A, S32.010B, S32.011A, S32.011B, S32.012A, S32.012B, S32.018A, S32.018B, S32.019A, S32.019B, S32.020A, S32.020B, S32.021A, S32.021B, S32.022A, S32.022B, S32.028A, S32.028B, S32.029A, S32.029B, S32.030A, S32.030B, S32.031A, S32.031B, S32.032A, S32.032B, S32.038A, S32.038B, S32.039A, S32.039B, S32.040A, S32.040B, S32.041A, S32.041B, S32.042A, S32.042B, S32.048A, S32.048B, S32.049A, S32.049B, S32.050A, S32.050B, S32.051A, S32.051B, S32.052A, S32.052B, S32.058A, S32.058B, S32.059A, S32.059B, S32.10XA, S32.10XB, S32.110A, S32.110B, S32.111A, S32.111B, S32.112A, S32.112B, S32.119A, S32.119B, S32.120A, S32.120B, S32.121A, S32.121B, S32.122A, S32.122B, S32.129A, S32.129B, S32.130A, S32.130B, S32.131A, S32.131B, S32.132A, S32.132B, S32.139A, S32.139B, S32.14XA, S32.14XB, S32.15XA, S32.15XB, S32.16XA, S32.16XB, S32.17XA, S32.17XB, S32.19XA, S32.19XB, S32.2XXA, S32.2XXB, S32.301A, S32.301B, S32.302A, S32.302B, S32.309A, S32.309B,S32.311A, S32.311B, S32.312A, S32.312B, S32.313A, S32.313B, S32.314A, S32.314B, S32.315A, S32.315B, S32.316A, S32.316B, S32.391A, S32.391B, S32.392A, S32.392B, S32.399A, S32.399B, S32.401A, S32.401B, S32.402A, S32.402B, S32.409A, S32.409B, S32.411A, S32.411B, S32.412A, S32.412B, S32.413A, S32.413B, S32.414A, S32.414B, S32.415A, S32.415B, S32.416A, S32.416B, S32.421A, S32.421B, S32.422A,S32.422B, S32.423A, S32.423B, S32.424A, S32.424B, S32.425A, S32.425B, S32.426A, S32.426B, S32.431A, S32.431B, S32.432A, S32.432B, S32.433A, S32.433B, S32.434A, S32.434B, S32.435A, S32.435B, S32.436A, S32.436B, S32.441A, S32.441B, S32.442A, S32.442B, S32.443A, S32.443B, S32.444A, S32.444B, S32.445A, S32.445B, S32.446A, S32.446B, S32.451A, S32.451B, S32.452A, S32.452B, S32.453A, S32.453B, S32.454A, S32.454B, S32.455A, S32.455B, S32.456A, S32.456B,

S32.461A, S32.461B, S32.462A, S32.462B, S32.463A, S32.463B, S32.464A, S32.464B, S32.465A, S32.465B, S32.466A, S32.466B, S32.471A, S32.471B, S32.472A, S32.472B, S32.473A, S32.473B, S32.474A, S32.474B, S32.475A, S32.475B, S32.476A, S32.476B, S32.481A, S32.481B, S32.482A, S32.482B, S32.483A, S32.483B, S32.484A, S32.484B, S32.485A, S32.485B, S32.486A, S32.486B, S32.491A, S32.491B, S32.492A, S32.492B, S32.499A, S32.499B, S32.501A, S32.501B, S32.502A, S32.502B, S32.509A, S32.509B, S32.511A, S32.511B, S32.512A, S32.512B, S32.519A, S32.519B, S32.591A, S32.591B, S32.592A, S32.592B, S32.599A, S32.599B, S32.601A, S32.601B, S32.602A, S32.602B, S32.609A, S32.609B, S32.611A, S32.611B, S32.612A, S32.612B, S32.613A, S32.613B, S32.614A, S32.614B, S32.615A, S32.615B, S32.616A, S32.616B, S32.691A, S32.691B, S32.692A, S32.692B, S32.699A, S32.699B, S32.810A, S32.810B, S32.811A, S32.811B, S32.82XA, S32.82XB, S32.89XA, S32.89XB, S32.9XXA, S32.9XXB, S42.001A, S42.001B, S42.002A, S42.002B, S42.009A, S42.009B, S42.011A, S42.011B, S42.012A, S42.012B, S42.013A, S42.013B, S42.014A, S42.014B, S42.015A, S42.015B, S42.016A, S42.016B, S42.017A, S42.017B, S42.018A, S42.018B, S42.019A, S42.019B, S42.021A, S42.021B, S42.022A, S42.022B, S42.023A, S42.023B, S42.024A, S42.024B, S42.025A, S42.025B, S42.026A, S42.026B, S42.031A, S42.031B, S42.032A, S42.032B, S42.033A, S42.033B, S42.034A, S42.034B, S42.035A, S42.035B, S42.036A, S42.036B, S42.101A, S42.101B, S42.102A, S42.102B, S42.109A, S42.109B, S42.111A, S42.111B, S42.112A, S42.112B, S42.113A, S42.113B, S42.114A, S42.114B, S42.115A, S42.115B, S42.116A, S42.116B, S42.121A, S42.121B, S42.122A, S42.122B, S42.123A, S42.123B, S42.124A, S42.124B, S42.125A, S42.125B, S42.126A, S42.126B, S42.131A, S42.131B, S42.132A, S42.132B, S42.133A, S42.133B, S42.134A, S42.134B, S42.135A, S42.135B, S42.136A, S42.136B, S42.141A, S42.141B, S42.142A, S42.142B, S42.143A, S42.143B, S42.144A, S42.144B, S42.145A, S42.145B, S42.146A, S42.146B, S42.151A, S42.151B, S42.152A, S42.152B, S42.153A, S42.153B, S42.154A, S42.154B, S42.155A, S42.155B, S42.156A, S42.156B,

S42.191A, S42.191B, S42.192A, S42.192B, S42.199A, S42.199B, S42.201A, S42.201B, S42.202A, S42.202B, S42.209A, S42.209B, S42.211A, S42.211B, S42.212A, S42.212B, S42.213A, S42.213B, S42.214A, S42.214B, S42.215A, S42.215B, S42.216A, S42.216B, S42.221A, S42.221B, S42.222A, S42.222B, S42.223A, S42.223B, S42.224A, S42.224B, S42.225A, S42.225B, S42.226A, S42.226B, S42.231A, S42.231B, S42.232A, S42.232B, S42.239A, S42.239B, S42.241A, S42.241B, S42.242A, S42.242B, S42.249A, S42.249B, S42.251A, S42.251B, S42.252A, S42.252B, S42.253A, S42.253B, S42.254A, S42.254B, S42.255A, S42.255B, S42.256A, S42.256B, S42.261A, S42.261B, S42.262A, S42.262B, S42.263A, S42.263B, S42.264A, S42.264B, S42.265A, S42.265B, S42.266A, S42.266B, S42.271A, S42.272A, S42.279A, S42.291A, S42.291B, S42.292A, S42.292B, S42.293A, S42.293B, S42.294A, S42.294B, S42.295A, S42.295B, S42.296A, S42.296B, S42.301A, S42.301B, S42.302A, S42.302B, S42.309A, S42.309B, , S42.321A, S42.321B, S42.322A, S42.322B, S42.323A, S42.323B, S42.324A, S42.324B, S42.325A, S42.325B, S42.326A, S42.326B, S42.331A, S42.331B, S42.332A, S42.332B, S42.333A, S42.333B, S42.334A, S42.334B, S42.335A, S42.335B, S42.336A, S42.336B, S42.341A, S42.341B, S42.342A, S42.342B, S42.343A, S42.343B, S42.344A, S42.344B, S42.345A, S42.345B, S42.346A, S42.346B, S42.351A, S42.351B, S42.352A, S42.352B, S42.353A, S42.353B, S42.354A, S42.354B, S42.355A, S42.355B, S42.356A, S42.356B, S42.361A, S42.361B, S42.362A, S42.362B, S42.363A, S42.363B, S42.364A, S42.364B, S42.365A, S42.365B, S42.366A, S42.366B, S42.391A, S42.391B, S42.392A, S42.392B, S42.399A, S42.399B, S42.401A, S42.401B, S42.402A, S42.402B, S42.409A, S42.409B, S42.411A, S42.411B, S42.412A, S42.412B, S42.413A, S42.413B, S42.414A, S42.414B, S42.415A, S42.415B, S42.416A, S42.416B, S42.421A, S42.421B, S42.422A, S42.422B, S42.423A, S42.423B, S42.424A, S42.424B, S42.425A, S42.425B, S42.426A, S42.426B, S42.431A, S42.431B, S42.432A, S42.432B, S42.433A, S42.433B, S42.434A, S42.434B, S42.435A, S42.435B, S42.436A, S42.436B, S42.441A, S42.441B,S42.442A, S42.442B, S42.443A, S42.443B, S42.444A,

S42.444B, S42.445A, S42.445B, S42.446A, S42.446B, S42.447A, S42.447B, S42.448A, S42.448B, S42.449A, S42.449B, S42.451A, S42.451B, S42.452A, S42.452B, S42.453A, S42.453B, S42.454A, S42.454B, S42.455A, S42.455B, S42.456A, S42.456B, S42.461A, S42.461B, S42.462A, S42.462B, S42.463A, S42.463B, S42.464A, S42.464B, S42.465A, S42.465B, S42.466A, S42.466B, S42.471A, S42.471B, S42.472A, S42.472B, S42.473A, S42.473B, S42.474A, S42.474B, S42.475A, S42.475B, S42.476A, S42.476B, S42.481A, S42.482A, S42.489A, S42.491A, S42.491B, S42.492A, S42.492B, S42.493A, S42.493B, S42.494A, S42.494B, S42.495A, S42.495B, S42.496A, S42.496B, S42.90XA, S42.90XB, S42.91XA, S42.91XB, S42.92XA, S42.92XB, S52.001A, S52.001B, S52.001C, S52.002A, S52.002B, S52.002C, S52.009A, S52.009B, S52.009C, S52.011A, S52.012A, S52.019A, S52.021A, S52.021B, S52.021C, S52.022A, S52.022B, S52.022C, S52.023A, S52.023B, S52.023C, S52.024A, S52.024B, S52.024C, S52.025A, S52.025B, S52.025C, S52.026A, S52.026B, S52.026C, S52.031A, S52.031B, S52.031C, S52.032A, S52.032B, S52.032C, S52.033A, S52.033B, S52.033C, S52.034A, S52.034B, S52.034C, S52.035A, S52.035B, S52.035C, S52.036A, S52.036B, S52.036C, S52.041A, S52.041B, S52.041C, S52.042A, S52.042B, S52.042C, S52.043A, S52.043B, S52.043C, S52.044A, S52.044B, S52.044C, S52.045A, S52.045B, S52.045C, S52.046A, S52.046B, S52.046C, S52.091A, S52.091B, S52.091C, S52.092A, S52.092B, S52.092C, S52.099A, S52.099B, S52.099C, S52.101A, S52.101B, S52.101C, S52.102A, S52.102B, S52.102C, S52.109A, S52.109B, S52.109C, S52.111A, S52.112A, S52.119A, S52.121A, S52.121B, S52.121C, S52.122A, S52.122B, S52.122C, S52.123A, S52.123B, S52.123C, S52.124A, S52.124B, S52.124C, S52.125A, S52.125B, S52.125C, S52.126A, S52.126B, S52.126C, S52.131A, S52.131B, S52.131C, S52.132A, S52.132B, S52.132C, S52.133A, S52.133B, S52.133C, S52.134A, S52.134B, S52.134C, S52.135A, S52.135B, S52.135C, S52.136A, S52.136B, S52.136C, S52.181A, S52.181B, S52.181C, S52.182A, S52.182B, S52.182C, S52.189A, S52.189B, S52.189C, S52.201A, S52.201B, S52.201C, S52.202A, S52.202B, S52.202C, S52.209A, S52.209B,

S52.209C, S52.221A, S52.221B, S52.221C, S52.222A, S52.222B, S52.222C, S52.223A, S52.223B, S52.223C, S52.224A, S52.224B, S52.224C, S52.225A, S52.225B, S52.225C, S52.226A, S52.226B, S52.226C, S52.231A, S52.231B, S52.231C, S52.232A, S52.232B, S52.232C, S52.233A, S52.233B, S52.233C, S52.234A, S52.234B, S52.234C, S52.235A, S52.235B, S52.235C, S52.236A, S52.236B, S52.236C, S52.241A, S52.241B, S52.241C, S52.242A, S52.242B, S52.242C, S52.243A, S52.243B, S52.243C, S52.244A, S52.244B, S52.244C, S52.245A, S52.245B, S52.245C, S52.246A, S52.246B, S52.246C, S52.251A, S52.251B, S52.251C, S52.252A, S52.252B, S52.252C, S52.253A, S52.253B, S52.253C, S52.254A, S52.254B, S52.254C, S52.255A, S52.255B, S52.255C, S52.256A, S52.256B, S52.256C, S52.261A, S52.261B, S52.261C, S52.262A, S52.262B, S52.262C, S52.263A, S52.263B, S52.263C, S52.264A, S52.264B, S52.264C, S52.265A, S52.265B, S52.265C, S52.266A, S52.266B, S52.266C, S52.271A, S52.271B, S52.271C, S52.272A, S52.272B, S52.272C, S52.279A, S52.279B, S52.279C, S52.281A, S52.281B, S52.281C, S52.282A, S52.282B, S52.282C, S52.283A, S52.283B, S52.283C, S52.291A, S52.291B, S52.291C, S52.292A, S52.292B, S52.292C, S52.299A, S52.299B, S52.299C, S52.301A, S52.301B, S52.301C, S52.302A, S52.302B, S52.302C, S52.309A, S52.309B, S52.309C, S52.321A, S52.321B, S52.321C, S52.322A, S52.322B, S52.322C, S52.323A, S52.323B, S52.323C, S52.324A, S52.324B, S52.324C, S52.325A, S52.325B, S52.325C, S52.326A, S52.326B, S52.326C, S52.331A, S52.331B, S52.331C, S52.332A, S52.332B, S52.332C, S52.333A, S52.333B, S52.333C, S52.334A, S52.334B, S52.334C, S52.335A, S52.335B, S52.335C, S52.336A, S52.336B, S52.336C, S52.341A, S52.341B, S52.341C, S52.342A, S52.342B, S52.342C, S52.343A, S52.343B, S52.343C, S52.344A, S52.344B, S52.344C, S52.345A, S52.345B, S52.345C, S52.346A, S52.346B, S52.346C, S52.351A, S52.351B, S52.351C, S52.352A, S52.352B, S52.352C, S52.353A, S52.353B, S52.353C, S52.354A, S52.354B, S52.354C, S52.355A, S52.355B,S52.355C, S52.356A, S52.356B, S52.356C, S52.361A, S52.361B, S52.361C, S52.362A, S52.362B, S52.362C, S52.363A, S52.363B, S52.363C,

S52.364A, S52.364B, S52.364C, S52.365A, S52.365B, S52.365C, S52.366A, S52.366B, S52.366C, S52.371A, S52.371B, S52.371C, S52.372A, S52.372B, S52.372C, S52.379A, S52.379B, S52.379C, S52.381A, S52.381B, S52.381C, S52.382A, S52.382B, S52.382C, S52.389A, S52.389B, S52.389C, S52.391A, S52.391B, S52.391C, S52.392A, S52.392B, S52.392C, S52.399A, S52.399B, S52.399C, S52.501A, S52.501B, S52.501C, S52.502A, S52.502B, S52.502C, S52.509A, S52.509B, S52.509C, S52.511A, S52.511B, S52.511C, S52.512A, S52.512B, S52.512C, S52.513A, S52.513B, S52.513C, S52.514A, S52.514B, S52.514C, S52.515A, S52.515B, S52.515C, S52.516A, S52.516B, S52.516C, S52.521A, S52.522A, S52.529A, S52.531A, S52.531B,S52.531C, S52.532A, S52.532B, S52.532C, S52.539A, S52.539B, S52.539C, S52.541A,S52.541B, S52.541C, S52.542A, S52.542B, S52.542C, S52.549A, S52.549B, S52.549C, S52.551A, S52.551B, S52.551C, S52.552A, S52.552B, S52.552C, S52.559A, S52.559B, S52.559C, S52.561A, S52.561B, S52.561C, S52.562A, S52.562B, S52.562C, S52.569A, S52.569B, S52.569C, S52.571A, S52.571B, S52.571C, S52.572A, S52.572B, S52.572C, S52.579A, S52.579B, S52.579C, S52.591A, S52.591B, S52.591C, S52.592A, S52.592B, S52.592C, S52.599A, S52.599B, S52.599C, S52.601A, S52.601B, S52.601C, S52.602A, S52.602B, S52.602C, S52.609A, S52.609B, S52.609C, S52.611A, S52.611B, S52.611C, S52.612A, S52.612B, S52.612C, S52.613A, S52.613B, S52.613C, S52.614A, S52.614B, S52.614C, S52.615A, S52.615B, S52.615C, S52.616A, S52.616B, S52.616C, S52.621A, S52.622A, S52.629A, S52.691A, S52.691B, S52.691C, S52.692A, S52.692B, S52.692C, S52.699A, S52.699B, S52.699C, S52.90XA, S52.90XB, S52.90XC, S52.91XA, S52.91XB, S52.91XC, S52.92XA, S52.92XB, S52.92XC, S62.001A, S62.001B, S62.002A, S62.002B, S62.009A, S62.009B, S62.011A, S62.011B, S62.012A, S62.012B, S62.013A, S62.013B, S62.014A, S62.014B, S62.015A, S62.015B, S62.016A, S62.016B, S62.021A, S62.021B, S62.022A, S62.022B, S62.023A, S62.023B, S62.024A, S62.024B, S62.025A, S62.025B, S62.026A, S62.026B, S62.031A, S62.031B, S62.032A, S62.032B, S62.033A, S62.033B, S62.034A, S62.034B, S62.035A, S62.035B,

S62.036A, S62.036B, S62.101A, S62.101B, S62.102A, S62.102B, S62.109A, S62.109B, S62.111A, S62.111B, S62.112A, S62.112B, S62.113A, S62.113B, S62.114A, S62.114B, S62.115A, S62.115B, S62.116A, S62.116B, S62.121A, S62.121B, S62.122A, S62.122B, S62.123A, S62.123B, S62.124A, S62.124B, S62.125A, S62.125B, S62.126A, S62.126B, S62.131A, S62.131B, S62.132A, S62.132B, S62.133A, S62.133B, S62.134A, S62.134B, S62.135A, S62.135B, S62.136A, S62.136B, S62.141A, S62.141B, S62.142A, S62.142B, S62.143A, S62.143B, S62.144A, S62.144B, S62.145A, S62.145B, S62.146A, S62.146B, S62.151A, S62.151B, S62.152A, S62.152B, S62.153A, S62.153B, S62.154A, S62.154B, S62.155A, S62.155B, S62.156A, S62.156B, S62.161A, S62.161B, S62.162A, S62.162B, S62.163A, S62.163B, S62.164A, S62.164B, S62.165A, S62.165B, S62.166A, S62.166B, S62.171A, S62.171B, S62.172A, S62.172B, S62.173A, S62.173B, S62.174A, S62.174B, S62.175A, S62.175B, S62.176A, S62.176B, S62.181A, S62.181B, S62.182A, S62.182B, S62.183A, S62.183B, S62.184A, S62.184B, S62.185A, S62.185B, S62.186A, S62.186B, S62.201A, S62.201B, S62.202A, S62.202B, S62.209A, S62.209B, S62.211A, S62.211B, S62.212A, S62.212B, S62.213A, S62.213B, S62.221A, S62.221B, S62.222A, S62.222B, S62.223A, S62.223B, S62.224A, S62.224B, S62.225A, S62.225B, S62.226A, S62.226B, S62.231A, S62.231B, S62.232A, S62.232B, S62.233A, S62.233B, S62.234A, S62.234B, S62.235A, S62.235B, S62.236A, S62.236B, S62.241A, S62.241B, S62.242A, S62.242B, S62.243A, S62.243B, S62.244A, S62.244B, S62.245A, S62.245B, S62.246A, S62.246B, S62.251A, S62.251B, S62.252A, S62.252B, S62.253A, S62.253B, S62.254A, S62.254B, S62.255A, S62.255B, S62.256A, S62.256B, S62.291A, S62.291B, S62.292A, S62.292B, S62.299A, S62.299B, S62.300A, S62.300B, S62.301A, S62.301B, S62.302A, S62.302B, S62.303A, S62.303B, S62.304A, S62.304B, S62.305A, S62.305B, S62.306A, S62.306B, S62.307A, S62.307B, S62.308A, S62.308B, S62.309A, S62.309B, S62.310A, S62.310B, S62.311A, S62.311B, S62.312A, S62.312B, S62.313A, S62.313B, S62.314A, S62.314B, S62.315A, S62.315B, S62.316A, S62.316B, S62.317A, S62.317B, S62.318A, S62.318B,

S62.319A, S62.319B, S62.320A, S62.320B, S62.321A, S62.321B, S62.322A, S62.322B, S62.323A, S62.323B, S62.324A, S62.324B, S62.325A, S62.325B, S62.326A, S62.326B, S62.327A, S62.327B, S62.328A, S62.328B, S62.329A, S62.329B, S62.330A, S62.330B, S62.331A, S62.331B, S62.332A, S62.332B, S62.333A, S62.333B, S62.334A, S62.334B, S62.335A, S62.335B, S62.336A, S62.336B, S62.337A, S62.337B, S62.338A, S62.338B, S62.339A, S62.339B, S62.340A, S62.340B, S62.341A, S62.341B, S62.342A, S62.342B, S62.343A, S62.343B, S62.344A, S62.344B, S62.345A, S62.345B, S62.346A, S62.346B, S62.347A, S62.347B, S62.348A, S62.348B, S62.349A, S62.349B, S62.350A, S62.350B, S62.351A, S62.351B, S62.352A, S62.352B, S62.353A, S62.353B, S62.354A, S62.354B, S62.355A, S62.355B, S62.356A, S62.356B, S62.357A, S62.357B, S62.358A, S62.358B, S62.359A, S62.359B, S62.360A, S62.360B, S62.361A, S62.361B, S62.362A, S62.362B, S62.363A, S62.363B, S62.364A, S62.364B, S62.365A, S62.365B, S62.366A, S62.366B, S62.367A, S62.367B, S62.368A, S62.368B, S62.369A, S62.369B, S62.390A, S62.390B, S62.391A, S62.391B, S62.392A, S62.392B, S62.393A, S62.393B, S62.394A, S62.394B, S62.395A, S62.395B,S62.396A, S62.396B, S62.397A, S62.397B, S62.398A, S62.398B, S62.399A, S62.399B, S62.90XA, S62.90XB, S62.91XA, S62.91XB, S62.92XA, S62.92XB, S72.001A, S72.001B, S72.001C, S72.002A, S72.002B, S72.002C, S72.009A, S72.009B, S72.009C, S72.011A, S72.011B, S72.011C, S72.012A, S72.012B, S72.012C, S72.019A, S72.019B, S72.019C, S72.031A, S72.031B, S72.031C, S72.032A, S72.032B, S72.032C, S72.033A, S72.033B, S72.033C, S72.034A, S72.034B, S72.034C, S72.035A, S72.035B, S72.035C, S72.036A, S72.036B, S72.036C, S72.041A, S72.041B, S72.041C, S72.042A, S72.042B, S72.042C, S72.043A, S72.043B, S72.043C, S72.044A, S72.044B, S72.044C, S72.045A, S72.045B, S72.045C, S72.046A, S72.046B, S72.046C, S72.051A, S72.051B, S72.051C, S72.052A, S72.052B, S72.052C, S72.059A, S72.059B, S72.059C, S72.061A, S72.061B, S72.061C, S72.062A, S72.062B, S72.062C, S72.063A, S72.063B, S72.063C, S72.064A, S72.064B, S72.064C, S72.065A, S72.065B, S72.065C, S72.066A, S72.066B,

S72.066C, S72.091A, S72.091B, S72.091C, S72.092A, S72.092B, S72.092C, S72.099A, S72.099B, S72.099C, S72.101A, S72.101B, S72.101C, S72.102A, S72.102B, S72.102C, S72.109A, S72.109B, S72.109C, S72.111A, S72.111B, S72.111C, S72.112A, S72.112B, S72.112C, S72.113A, S72.113B, S72.113C, S72.114A, S72.114B, S72.114C, S72.115A, S72.115B, S72.115C, S72.116A, S72.116B, S72.116C, S72.121A, S72.121B, S72.121C, S72.122A, S72.122B, S72.122C, S72.123A, S72.123B, S72.123C, S72.124A, S72.124B, S72.124C, S72.125A, S72.125B, S72.125C, S72.126A, S72.126B, S72.126C, S72.141A, S72.141B, S72.141C, S72.142A, S72.142B, S72.142C, S72.143A, S72.143B, S72.143C, S72.144A, S72.144B, S72.144C, S72.145A, S72.145B, S72.145C, S72.146A, S72.146B, S72.146C, S72.21XA, S72.21XB, S72.21XC, S72.22XA, S72.22XB, S72.22XC, S72.23XA, S72.23XB, S72.23XC, S72.24XA, S72.24XB, S72.24XC, S72.25XA, S72.25XB, S72.25XC, S72.26XA, S72.26XB, S72.26XC, S72.301A, S72.301B, S72.301C, S72.302A, S72.302B, S72.302C, S72.309A, S72.309B, S72.309C, S72.321A, S72.321B, S72.321C, S72.322A, S72.322B, S72.322C, S72.323A, S72.323B, S72.323C, S72.324A, S72.324B, S72.324C, S72.325A, S72.325B, S72.325C, S72.326A, S72.326B, S72.326C, S72.331A, S72.331B, S72.331C, S72.332A, S72.332B, S72.332C, S72.333A, S72.333B, S72.333C, S72.334A, S72.334B, S72.334C, S72.335A, S72.335B, S72.335C, S72.336A, S72.336B, S72.336C, S72.341A, S72.341B, S72.341C, S72.342A, S72.342B, S72.342C, S72.343A, S72.343B, S72.343C, S72.344A, S72.344B, S72.344C, S72.345A, S72.345B, S72.345C, S72.346A, S72.346B, S72.346C, S72.351A, S72.351B, S72.351C, S72.352A, S72.352B, S72.352C, S72.353A, S72.353B, S72.353C, S72.354A, S72.354B, S72.354C, S72.355A, S72.355B, S72.355C, S72.356A, S72.356B, S72.356C, S72.361A, S72.361B, S72.361C, S72.362A, S72.362B, S72.362C, S72.363A, S72.363B, S72.363C, S72.364A, S72.364B, S72.364C, S72.365A, S72.365B, S72.365C, S72.366A, S72.366B, S72.366C, S72.391A, S72.391B, S72.391C, S72.392A, S72.392B, S72.392C, S72.399A, S72.399B, S72.399C, S72.401A, S72.401B, S72.401C, S72.402A, S72.402B, S72.402C, S72.409A, S72.409B, S72.409C,

S72.411A, S72.411B, S72.411C, S72.412A, S72.412B, S72.412C, S72.413A, S72.413B, S72.413C, S72.414A, S72.414B, S72.414C, S72.415A, S72.415B, S72.415C, S72.416A, S72.416B, S72.416C, S72.421A, S72.421B, S72.421C, S72.422A, S72.422B, S72.422C, S72.423A, S72.423B, S72.423C, S72.424A, S72.424B, S72.424C, S72.425A, S72.425B, S72.425C, S72.426A, S72.426B, S72.426C, S72.431A, S72.431B, S72.431C, S72.432A, S72.432B, S72.432C, S72.433A, S72.433B, S72.433C, S72.434A, S72.434B, S72.434C, S72.435A, S72.435B, S72.435C, S72.436A, S72.436B, S72.436C, S72.451A, S72.451B, S72.451C, S72.452A, S72.452B, S72.452C, S72.453A, S72.453B, S72.453C, S72.454A, S72.454B, S72.454C, S72.455A, S72.455B, S72.455C, S72.456A, S72.456B, S72.456C, S72.461A, S72.461B, S72.461C, S72.462A, S72.462B, S72.462C, S72.463A, S72.463B, S72.463C, S72.464A, S72.464B, S72.464C, S72.465A, S72.465B, S72.465C, S72.466A, S72.466B, S72.466C, S72.471A, S72.472A, S72.479A, S72.491A, S72.491B, S72.491C, S72.492A, S72.492B, S72.492C, S72.499A, S72.499B, S72.499C, S72.8X1A, S72.8X1B, S72.8X1C, S72.8X2A, S72.8X2B, S72.8X2C, S72.8X9A,S72.8X9B, S72.8X9C, S72.90XA, S72.90XB,S72.90XC, S72.91XA, S72.91XB, S72.91XC, S72.92XA, S72.92XB, S72.92XC, S82.001A, S82.001B, S82.001C, S82.002A, S82.002B, S82.002C, S82.009A, S82.009B, S82.009C, S82.011A, S82.011B, S82.011C, S82.012A, S82.012B, S82.012C, S82.013A, S82.013B, S82.013C, S82.014A, S82.014B, S82.014C, S82.015A, S82.015B, S82.015C, S82.016A, S82.016B, S82.016C, S82.021A, S82.021B, S82.021C, S82.022A, S82.022B, S82.022C, S82.023A, S82.023B, S82.023C, S82.024A, S82.024B, S82.024C, S82.025A, S82.025B, S82.025C, S82.026A, S82.026B, S82.026C, S82.031A, S82.031B, S82.031C, S82.032A, S82.032B, S82.032C, S82.033A, S82.033B, S82.033C, S82.034A, S82.034B, S82.034C, S82.035A, S82.035B, S82.035C, S82.036A, S82.036B, S82.036C, S82.041A, S82.041B, S82.041C, S82.042A, S82.042B, S82.042C, S82.043A, S82.043B, S82.043C, S82.044A, S82.044B, S82.044C, S82.045A, S82.045B, S82.045C, S82.046A, S82.046B, S82.046C, S82.091A, S82.091B, S82.091C, S82.092A, S82.092B, S82.092C, S82.099A,

S82.099B, S82.099C, S82.101A, S82.101B, S82.101C, S82.102A, S82.102B, S82.102C, S82.109A, S82.109B, S82.109C, S82.111A, S82.111B, S82.111C, S82.112A, S82.112B, S82.112C, S82.113A, S82.113B, S82.113C, S82.114A, S82.114B, S82.114C, S82.115A, S82.115B, S82.115C, S82.116A, S82.116B, S82.116C, S82.121A, S82.121B, S82.121C, S82.122A, S82.122B, S82.122C, S82.123A, S82.123B, S82.123C, S82.124A, S82.124B, S82.124C, S82.125A, S82.125B, S82.125C, S82.126A, S82.126B, S82.126C, S82.131A, S82.131B, S82.131C, S82.132A, S82.132B, S82.132C, S82.133A, S82.133B, S82.133C, S82.134A, S82.134B, S82.134C, S82.135A, S82.135B, S82.135C, S82.136A, S82.136B, S82.136C, S82.141A, S82.141B, S82.141C, S82.142A, S82.142B, S82.142C, S82.143A, S82.143B, S82.143C, S82.144A, S82.144B, S82.144C, S82.145A, S82.145B, S82.145C, S82.146A, S82.146B, S82.146C, S82.151A, S82.151B, S82.151C, S82.152A, S82.152B, S82.152C, S82.153A, S82.153B, S82.153C, S82.154A, S82.154B, S82.154C, S82.155A, S82.155B, S82.155C, S82.156A, S82.156B, S82.156C, S82.161A, S82.162A, S82.169A, S82.191A, S82.191B, S82.191C, S82.192A, S82.192B, S82.192C, S82.199A, S82.199B, S82.199C, S82.201A, S82.201B, S82.201C, S82.202A, S82.202B, S82.202C, S82.209A, S82.209B, S82.209C, S82.221A, S82.221B, S82.221C, S82.222A, S82.222B, S82.222C, S82.223A, S82.223B, S82.223C, S82.224A, S82.224B, S82.224C, S82.225A, S82.225B, S82.225C, S82.226A, S82.226B, S82.226C, S82.231A, S82.231B, S82.231C, S82.232A, S82.232B, S82.232C, S82.233A, S82.233B, S82.233C, S82.234A, S82.234B, S82.234C, S82.235A, S82.235B, S82.235C, S82.236A, S82.236B, S82.236C, S82.241A, S82.241B, S82.241C, S82.242A, S82.242B, S82.242C, S82.243A, S82.243B, S82.243C, S82.244A, S82.244B, S82.244C, S82.245A, S82.245B, S82.245C, S82.246A, S82.246B, S82.246C, S82.251A, S82.251B, S82.251C, S82.252A, S82.252B, S82.252C, S82.253A, S82.253B, S82.253C, S82.254A, S82.254B, S82.254C, S82.255A, S82.255B, S82.255C, S82.256A, S82.256B, S82.256C, S82.261A, S82.261B, S82.261C, S82.262A, S82.262B, S82.262C, S82.263A, S82.263B, S82.263C, S82.264A, S82.264B, S82.264C, S82.265A, S82.265B,

S82.265C, S82.266A, S82.266B, S82.266C, S82.291A, S82.291B, S82.291C, S82.292A, S82.292B, S82.292C, S82.299A, S82.299B, S82.299C, S82.301A, S82.301B, S82.301C, S82.302A, S82.302B, S82.302C, S82.309A, S82.309B, S82.309C, S82.311A, S82.312A, S82.319A, S82.391A, S82.391B, S82.391C, S82.392A, S82.392B, S82.392C, S82.399A, S82.399B, S82.399C, S82.401A, S82.401B, S82.401C, S82.402A, S82.402B, S82.402C, S82.409A, S82.409B, S82.409C, S82.421A, S82.421B, S82.421C, S82.422A, S82.422B, S82.422C, S82.423A, S82.423B, S82.423C, S82.424A, S82.424B, S82.424C, S82.425A, S82.425B, S82.425C, S82.426A, S82.426B, S82.426C, S82.431A, S82.431B, S82.431C, S82.432A, S82.432B, S82.432C, S82.433A, S82.433B, S82.433C, S82.434A, S82.434B, S82.434C, S82.435A, S82.435B, S82.435C, S82.436A, S82.436B, S82.436C, S82.441A, S82.441B, S82.441C, S82.442A, S82.442B, S82.442C, S82.443A, S82.443B, S82.443C, S82.444A, S82.444B, S82.444C, S82.445A, S82.445B, S82.445C, S82.446A, S82.446B, S82.446C, S82.451A, S82.451B, S82.451C, S82.452A, S82.452B, S82.452C, S82.453A, S82.453B, S82.453C, S82.454A, S82.454B, S82.454C, S82.455A, S82.455B, S82.455C, S82.456A, S82.456B, S82.456C, S82.461A, S82.461B, S82.461C, S82.462A, S82.462B, S82.462C, S82.463A, S82.463B, S82.463C, S82.464A, S82.464B, S82.464C, S82.465A, S82.465B, S82.465C, S82.466A, S82.466B, S82.466C, S82.491A,S82.491B, S82.491C, S82.492A, S82.492B, S82.492C, S82.499A,S82.499B, S82.499C, S82.51XA, S82.51XB, S82.51XC, S82.52XA, S82.52XB, S82.52XC, S82.53XA, S82.53XB, S82.53XC, S82.54XA, S82.54XB, S82.54XC, S82.55XA, S82.55XB, S82.55XC, S82.56XA, S82.56XB, S82.56XC, S82.61XA, S82.61XB, S82.61XC, S82.62XA, S82.62XB, S82.62XC, S82.63XA, S82.63XB, S82.63XC, S82.64XA, S82.64XB, S82.64XC, S82.65XA, S82.65XB, S82.65XC, S82.66XA, S82.66XB, S82.66XC, S82.811A, S82.812A, S82.819A, S82.821A, S82.822A, S82.829A, S82.831A, S82.831B, S82.831C, S82.832A, S82.832B, S82.832C, S82.839A, S82.839B, S82.839C, S82.841A, S82.841B, S82.841C, S82.842A, S82.842B, S82.842C, S82.843A, S82.843B, S82.843C, S82.844A, S82.844B, S82.844C, S82.845A, S82.845B, S82.845C,

S82.846A, S82.846B, S82.846C, S82.851A, S82.851B, S82.851C, S82.852A, S82.852B, S82.852C, S82.853A, S82.853B, S82.853C, S82.854A, S82.854B, S82.854C, S82.855A, S82.855B, S82.855C, S82.856A, S82.856B, S82.856C, S82.861A, S82.861B, S82.861C, S82.862A, S82.862B, S82.862C, S82.863A, S82.863B, S82.863C, S82.864A, S82.864B, S82.864C, S82.865A, S82.865B, S82.865C, S82.866A, S82.866B, S82.866C, S82.871A, S82.871B, S82.871C, S82.872A, S82.872B, S82.872C, S82.873A, S82.873B, S82.873C, S82.874A, S82.874B, S82.874C, S82.875A, S82.875B, S82.875C, S82.876A, S82.876B, S82.876C, S82.891A, S82.891B, S82.891C, S82.892A, S82.892B, S82.892C, S82.899A, S82.899B, S82.899C, S82.90XA, S82.90XB, S82.90XC, S82.91XA, S82.91XB, S82.91XC, S82.92XA, S82.92XB, S82.92XC, S92.001A, S92.001B, S92.002A, S92.002B, S92.009A, S92.009B, S92.011A, S92.011B, S92.012A, S92.012B, S92.013A, S92.013B, S92.014A, S92.014B, S92.015A, S92.015B, S92.016A, S92.016B, S92.021A, S92.021B, S92.022A, S92.022B, S92.023A, S92.023B, S92.024A, S92.024B, S92.025A, S92.025B, S92.026A, S92.026B, S92.031A, S92.031B, S92.032A, S92.032B, S92.033A, S92.033B, S92.034A, S92.034B, S92.035A, S92.035B, S92.036A, S92.036B, S92.041A, S92.041B, S92.042A, S92.042B, S92.043A, S92.043B, S92.044A, S92.044B, S92.045A, S92.045B, S92.046A, S92.046B, S92.051A, S92.051B, S92.052A, S92.052B, S92.053A, S92.053B, S92.054A, S92.054B, S92.055A, S92.055B, S92.056A, S92.056B, S92.061A, S92.061B, S92.062A, S92.062B, S92.063A, S92.063B, S92.064A, S92.064B, S92.065A, S92.065B, S92.066A, S92.066B, S92.101A, S92.101B, S92.102A, S92.102B, S92.109A, S92.109B, S92.111A, S92.111B, S92.112A, S92.112B, S92.113A, S92.113B, S92.114A, S92.114B, S92.115A, S92.115B, S92.116A, S92.116B, S92.121A, S92.121B, S92.122A, S92.122B, S92.123A, S92.123B, S92.124A, S92.124B, S92.125A, S92.125B,S92.126A, S92.126B, S92.131A, S92.131B, S92.132A, S92.132B, S92.133A, S92.133B, S92.134A,S92.134B, S92.135A, S92.135B, S92.136A, S92.136B, S92.141A, S92.141B, S92.142A, S92.142B, S92.143A, S92.143B, S92.144A, S92.144B, S92.145A, S92.145B, S92.146A, S92.146B, S92.151A,

S92.151B, S92.152A,S92.152B, S92.153A, S92.153B, S92.154A, S92.154B, S92.155A, S92.155B, S92.156A, S92.156B,S92.191A, S92.191B, S92.192A, S92.192B, S92.199A, S92.199B, S92.201A, S92.201B, S92.202A,S92.202B, S92.209A, S92.209B, S92.211A, S92.211B, S92.212A, S92.212B, S92.213A, S92.213B,S92.214A, S92.214B, S92.215A, S92.215B, S92.216A, S92.216B, S92.221A, S92.221B, S92.222A, S92.222B, S92.223A, S92.223B, S92.224A, S92.224B, S92.225A, S92.225B, S92.226A, S92.226B, S92.231A, S92.231B, S92.232A, S92.232B, S92.233A, S92.233B, S92.234A, S92.234B, S92.235A, S92.235B, S92.236A, S92.236B, S92.241A, S92.241B, S92.242A, S92.242B, S92.243A, S92.243B,S92.244A, S92.244B, S92.245A, S92.245B, S92.246A, S92.246B, S92.251A, S92.251B, S92.252A,S92.252B, S92.253A, S92.253B, S92.254A, S92.254B, S92.255A, S92.255B, S92.256A, S92.256B,S92.301A, S92.301B, S92.302A, S92.302B, S92.309A, S92.309B, S92.311A, S92.311B, S92.312A, S92.312B, S92.313A, S92.313B, S92.314A, S92.314B, S92.315A, S92.315B, S92.316A, S92.316B, S92.321A, S92.321B, S92.322A, S92.322B, S92.323A, S92.323B, S92.324A, S92.324B, S92.325A,S92.325B, S92.326A, S92.326B, S92.331A, S92.331B, S92.332A, S92.332B, S92.333A, S92.333B,S92.334A, S92.334B, S92.335A, S92.335B, S92.336A, S92.336B, S92.341A, S92.341B, S92.342A, S92.342B, S92.343A, S92.343B, S92.344A, S92.344B, S92.345A, S92.345B, S92.346A, S92.346B,S92.351A, S92.351B, S92.352A, S92.352B, S92.353A, S92.353B, S92.354A, S92.354B, S92.355A, S92.355B, S92.356A, S92.356B, S92.811A, S92.811B, S92.812A, S92.812B, S92.819A, S92.819B, S92.901A, S92.901B, S92.902A, S92.902B, S92.909A, S92.909B

### 1.2.2 Osteoarthritis ICD codes

ICD-9 Codes: 715.15, 716.16, 715.11.

ICD-10 Codes:

M15.0, M15.1, M15.2, M15.3, M15.4, M15.8, M15.9,M16.0, M16.10, M16.11, M16.12, M16.2, M16.30, M16.31, M16.32, M16.4, M16.50, M16.51, M16.52,M16.6, M16.7, M16.9, M17.0, M17.10, M17.11, M17.12, M17.2, M17.30, M17.31, M17.32, M17.4, M17.5,M17.9, M18.0, M18.10, M18.11, M18.12, M18.2, M18.30, M18.31, M18.32, M18.4, M18.50, M18.51,M18.52, M18.9, M19.011, M19.012, M19.019, M19.021, M19.022, M19.029, M19.031, M19.032, M19.039,M19.041, M19.042, M19.049, M19.071, M19.072, M19.079, M19.111, M19.112, M19.119, M19.121,M19.122, M19.129, M19.131, M19.132, M19.139, M19.141, M19.142, M19.149, M19.171, M19.172,M19.179, M19.211, M19.212, M19.219, M19.221, M19.222, M19.229, M19.231, M19.232, M19.239,M19.241, M19.242, M19.249, M19.271, M19.272, M19.279, M19.90, M19.91, M19.92, M19.93

### 1.2.3 Osteoporosis ICD codes

ICD-9 Codes: 733.01, 733.00, 733.02, 733.03, 733.09.

ICD-10 Codes:

M80.00XA, M80.00XD, M80.00XG, M80.00XK, M80.00XP, M80.00XS, M80.011A, M80.011D, M80.011G, M80.011K, M80.011P, M80.011S, M80.012A, M80.012D, M80.012G, M80.012K, M80.012P, M80.012S, M80.019A, M80.019D, M80.019G, M80.019K, M80.019P, M80.019S, M80.021A, M80.021D, M80.021G, M80.021K, M80.021P, M80.021S, M80.022A, M80.022D, M80.022G, M80.022K, M80.022P, M80.022S, M80.029A, M80.029D, M80.029G, M80.029K, M80.029P, M80.029S, M80.031A, M80.031D, M80.031G, M80.031K, M80.031P, M80.031S, M80.032A, M80.032D, M80.032G, M80.032K, M80.032P, M80.032S, M80.039A, M80.039D, M80.039G, M80.039K, M80.039P, M80.039S, M80.041A, M80.041D, M80.041G, M80.041K, M80.041P, M80.041S, M80.042A, M80.042D, M80.042G, M80.042K, M80.042P, M80.042S, M80.049A, M80.049D, M80.049G, M80.049K, M80.049P, M80.049S, M80.051A, M80.051D, M80.051G, M80.051K, M80.051P, M80.051S, M80.052A, M80.052D, M80.052G,

M80.052K, M80.052P, M80.052S, M80.059A, M80.059D, M80.059G, M80.059K, M80.059P, M80.059S, M80.061A, M80.061D, M80.061G, M80.061K, M80.061P, M80.061S, M80.062A, M80.062D, M80.062G, M80.062K, M80.062P, M80.062S, M80.069A, M80.069D, M80.069G, M80.069K, M80.069P, M80.069S, M80.071A, M80.071D, M80.071G, M80.071K, M80.071P, M80.071S, M80.072A, M80.072D, M80.072G, M80.072K, M80.072P, M80.072S, M80.079A, M80.079D, M80.079G, M80.079K, M80.079P, M80.079S, M80.08XA, M80.08XD, M80.08XG, M80.08XK, M80.08XP, M80.08XS, M80.80XA, M80.80XD, M80.80XG, M80.80XK, M80.80XP, M80.80XS, M80.811A, M80.811D, M80.811G, M80.811K, M80.811P, M80.811S, M80.812A, M80.812D, M80.812G, M80.812K, M80.812P, M80.812S, M80.819A, M80.819D, M80.819G, M80.819K, M80.819P, M80.819S, M80.821A, M80.821D, M80.821G, M80.821K, M80.821P, M80.821S, M80.822A, M80.822D, M80.822G, M80.822K, M80.822P, M80.822S, M80.829A, M80.829D, M80.829G, M80.829K, M80.829P, M80.829S, M80.831A, M80.831D, M80.831G, M80.831K, M80.831P, M80.831S, M80.832A, M80.832D, M80.832G, M80.832K, M80.832P, M80.832S, M80.839A, M80.839D, M80.839G, M80.839K, M80.839P, M80.839S, M80.841A, M80.841D, M80.841G, M80.841K, M80.841P, M80.841S, M80.842A, M80.842D, M80.842G, M80.842K, M80.842P, M80.842S, M80.849A, M80.849D, M80.849G, M80.849K, M80.849P, M80.849S, M80.851A, M80.851D, M80.851G,M80.851K, M80.851P, M80.851S, M80.852A, M80.852D, M80.852G, M80.852K, M80.852P, M80.852S, M80.859A, M80.859D, M80.859G, M80.859K, M80.859P, M80.859S, M80.861A, M80.861D, M80.861G, M80.861K, M80.861P, M80.861S, M80.862A, M80.862D, M80.862G, M80.862K, M80.862P, M80.862S, M80.869A, M80.869D, M80.869G, M80.869K, M80.869P, M80.869S, M80.871A, M80.871D, M80.871G, M80.871K, M80.871P, M80.871S, M80.872A, M80.872D, M80.872G, M80.872K, M80.872P, M80.872S, M80.879A, M80.879D, M80.879G, M80.879K, M80.879P, M80.879S, M80.88XA, M80.88XD, M80.88XG, M80.88XK, M80.88XP, M80.88XS, M81.0, M81.6, M81.8

# 2 Patient demographics

See Table 1 for the demographics of our patient cohort.

Table 1: Demographics of the patient cohort.

| | **Readmission (N=255)** | **No (N=947)** | **Overall (N=1,202)** |
|---|---|---|---|
| **Age** | | | |
| Mean (SD) | 69.2 (9.97) | 65.4 (9.13) | 66.3 (9.43) |
| Median [Min, Max] | 69.0 [50.0, 96.0] | 65.0 [50.0, 92.0] | 66.0 [50.0, 96.0] |
| **Elixhauser comorbidity score** | | | |
| Mean (SD) | 9.09 (9.62) | 4.36 (6.93) | 5.36 (7.82) |
| Median [Min, Max] | 7.00 [-2.00, 46.0] | 2.00 [-2.00, 67.0] | 2.50 [-2.00, 67.0] |
| **Sex** | | | |
| Male | 57 (22.4%) | 215 (22.7%) | 272 (22.6%) |
| Female | 198 (77.6%) | 732 (77.3%) | 930 (77.4%) |
| **Race** | | | |
| White | 213 (83.5%) | 807 (85.2%) | 1020 (84.9%) |
| Black | 39 (15.3%) | 98 (10.3%) | 137 (11.4%) |
| Other | 3 (1.2%) | 42 (4.4%) | 45 (3.7%) |
| **With partner** | | | |
| Yes | 115 (45.1%) | 578 (61.0%) | 693 (57.7%) |
| No | 140 (54.9%) | 369 (39.0%) | 509 (42.3%) |
| **Smoking** | | | |
| Never | 129 (50.6%) | 559 (59.0%) | 688 (57.2%) |
| Former | 104 (40.8%) | 316 (33.4%) | 420 (34.9%) |
| Current | 22 (8.6%) | 72 (7.6%) | 94 (7.8%) |
| **Insurance** | | | |
| Government | 188 (73.7%) | 480 (50.7%) | 668 (55.6%) |
| Commercial | 59 (23.1%) | 398 (42.0%) | 457 (38.0%) |
| WCSC | 5 (2.0%) | 39 (4.1%) | 44 (3.7%) |
| Self-pay | 3 (1.2%) | 30 (3.2%) | 33 (2.7%) |

# 3 Insurance type

Here is how we grouped insurance types based on information from the raw EHR data:

1. Government Insurance:
   - Medicare

- Medicare Advantage
- NC MEDICAID
- NS Medicaid Managed Care
- Medicaid Pending
- OOS Medicaid
- Other Government

2. Commercial Insurance:
    - Managed Care
    - NC Blue Cross
    - OOS Blue Cross
    - Commercial
3. Worker's Compensation and Specialized Coverage:
    - Worker's Comp
    - Liability
    - Special Programs
4. Self-Pay and Uninsured

# 4 Kriging under the Hilbert space Gaussian process approximation

In this section, we show that if $m \leq n$ under the Hilbert space Gaussian process (HSGP) approximation, the kriging distribution is necessarily degenerate, with $\boldsymbol{\theta}^*_{0j} \mid \boldsymbol{\theta}_{0j}, \boldsymbol{\Omega} = (\boldsymbol{\Phi}^*\mathbf{S}\boldsymbol{\Phi}^\top)(\boldsymbol{\Phi}\mathbf{S}\boldsymbol{\Phi}^\top)^+\boldsymbol{\theta}_{0j}$, where $\mathbf{A}^+$ denote a generalized inverse of matrix $\mathbf{A}$. For simplicity of notation, we will drop the subscripts and use $\boldsymbol{\theta}$ and $\boldsymbol{\theta}^*$ from now on.

First, we state an established result for multivariate normal distributions. Let $\mathbf{X}_a$ and $\mathbf{X}_b$ be two random vectors, jointly multivariate normal,

$$\begin{pmatrix} \mathbf{X}_a \\ \mathbf{X}_b \end{pmatrix} \sim N\left(\begin{pmatrix} \boldsymbol{\mu}_a \\ \boldsymbol{\mu}_b \end{pmatrix}, \boldsymbol{\Sigma} = \begin{pmatrix} \boldsymbol{\Sigma}_{aa} & \boldsymbol{\Sigma}_{ab} \\ \boldsymbol{\Sigma}_{ba} & \boldsymbol{\Sigma}_{bb} \end{pmatrix}\right),$$

where $\boldsymbol{\Sigma}$ can be singular. The conditional distribution of $\mathbf{X}_a \mid \mathbf{X}_b = \mathbf{x}_b$ is $N(\mathbf{d}, \boldsymbol{\Psi})$, where

$$\mathbf{d} = \boldsymbol{\mu}_a + \boldsymbol{\Sigma}_{ab}\boldsymbol{\Sigma}_{bb}^+\mathbf{x}_b, \quad \boldsymbol{\Psi} = \boldsymbol{\Sigma}_{aa} - \boldsymbol{\Sigma}_{ab}\boldsymbol{\Sigma}_{bb}^+\boldsymbol{\Sigma}_{ba}.$$

Therefore the kriging distribution under HSGP is $\boldsymbol{\theta}^* \mid \boldsymbol{\theta} \sim N(\mathbf{d}, \boldsymbol{\Psi})$, with

$$\mathbf{d} = (\boldsymbol{\Phi}^*\mathbf{S}\boldsymbol{\Phi}^\top)(\boldsymbol{\Phi}\mathbf{S}\boldsymbol{\Phi}^\top)^+\boldsymbol{\theta}, \quad \boldsymbol{\Psi} = (\boldsymbol{\Phi}^*\mathbf{S}\boldsymbol{\Phi}^{*\top}) - (\boldsymbol{\Phi}^*\mathbf{S}\boldsymbol{\Phi}^\top)(\boldsymbol{\Phi}\mathbf{S}\boldsymbol{\Phi}^\top)^+(\boldsymbol{\Phi}\mathbf{S}\boldsymbol{\Phi}^{*\top}).$$

If $m > n$, $(\boldsymbol{\Phi}\mathbf{S}\boldsymbol{\Phi}^\top)$ is invertible, hence $(\boldsymbol{\Phi}\mathbf{S}\boldsymbol{\Phi}^\top)^+ = (\boldsymbol{\Phi}\mathbf{S}\boldsymbol{\Phi}^\top)^{-1}$, and the kriging distribution is the multivariate normal stated in the article; If $m \leq n$, we will show that the kriging distribution is necessarily degenerate, i.e., $\boldsymbol{\Psi} \equiv 0$. This is equivalent to showing

$$(\boldsymbol{\Phi}^*\mathbf{S}\boldsymbol{\Phi}^{*\top}) = (\boldsymbol{\Phi}^*\mathbf{S}\boldsymbol{\Phi}^\top)(\boldsymbol{\Phi}\mathbf{S}\boldsymbol{\Phi}^\top)^+(\boldsymbol{\Phi}\mathbf{S}\boldsymbol{\Phi}^{*\top}).$$

It's also equivalent to showing $\mathbf{S} = \mathbf{S}\boldsymbol{\Phi}^\top(\boldsymbol{\Phi}\mathbf{S}\boldsymbol{\Phi}^\top)^+\boldsymbol{\Phi}\mathbf{S}$. Note that under HSGP, if $m \leq n$, the $n \times m$ feature matrix $\boldsymbol{\Phi}$ has full column rank. Therefore for all $\mathbf{x}, \mathbf{y} \in \mathbb{R}^m$,

$$\boldsymbol{\Phi}\mathbf{x} = \boldsymbol{\Phi}\mathbf{y} \implies \mathbf{x} = \mathbf{y}, \quad \mathbf{x}^\top\boldsymbol{\Phi}^\top = \mathbf{y}^\top\boldsymbol{\Phi}^\top \implies \mathbf{x} = \mathbf{y}. \tag{1}$$

By the definition of generalized inverse, $(\mathbf{\Phi S \Phi}^\top)(\mathbf{\Phi S \Phi}^\top)^+(\mathbf{\Phi S \Phi}^\top) = (\mathbf{\Phi S \Phi}^\top)$. Now applying equation (1), we have

$$\mathbf{S\Phi}^\top(\mathbf{\Phi S \Phi}^\top)^+\mathbf{\Phi S} = \mathbf{S}. \tag{2}$$

which is exactly what's needed to show $\mathbf{\Psi} \equiv \mathbf{0}$ as argued above. If we use a non-centered parameterization in `Stan`, and set $\boldsymbol{\theta} = \mathbf{\Phi S}^{1/2}\mathbf{z}$ for $\mathbf{z} \sim N_m(0, I)$, then the conditional mean $\mathbf{d} = (\mathbf{\Phi}^*\mathbf{S\Phi}^\top)(\mathbf{\Phi S \Phi}^\top)^+\mathbf{\Phi S}^{1/2}\mathbf{z}$. Plugging in equation (2) and using the fact that $\mathbf{S}$ is invertible, we have $\mathbf{d} = \mathbf{\Phi}^*\mathbf{S}^{1/2}\mathbf{z}$.

# 5 Additional results for the simulation study

In this section we present additional simulation study results. First, see Table 2 for RMSE of the regression coefficients for risk type 2.

Table 2: Risk type 2 regression coefficients RMSE from simulation study.

| Model | $\beta_{1,1}$ | $\beta_{2,1}$ | $\beta_{3,1}$ | $\beta_{4,1}$ | $\beta_{5,1}$ | $\beta_{6,1}$ | $\beta_{7,1}$ | $\beta_{8,1}$ | $\beta_{9,1}$ | $\beta_{10,1}$ | $\beta_{w,1}$ |
|---|---|---|---|---|---|---|---|---|---|---|---|
| Coxph | 0.45 | 1.47 | 0.28 | 0.25 | 0.59 | 0.26 | 0.34 | 0.93 | 1.27 | 0.17 | 0.32 |
| Coxph+groups | 0.45 | 1.50 | 0.31 | 0.27 | 0.62 | 0.28 | 0.38 | 0.96 | 1.35 | 0.19 | 0.44 |
| BSp GP | 0.35 | 0.42 | 0.22 | 0.20 | 0.29 | 0.20 | 0.24 | 0.30 | 0.47 | 0.13 | 0.30 |
| BSp HSGP | 0.35 | 0.41 | 0.22 | 0.20 | 0.29 | 0.20 | 0.23 | 0.30 | 0.47 | 0.13 | 0.28 |

Figure 1 presents the distribution of the RMSEs of the piecewise-constant baseline hazard rates across simulated datasets. For ease of comparison, the y-axis was capped at 2, although some RMSE values were much larger. Figure 2 presents the posterior means of the piecewise-constant baseline hazard rates for risk type 2 from the simulated datasets, compared to the true curve. Figures 3 and 4 present the posterior means and posterior standard deviation results for risk type 2. Figure 5 presents averages of RMSEs of the spatial surfaces. Figure 6 presents the posterior coverage for the spatial surfaces.

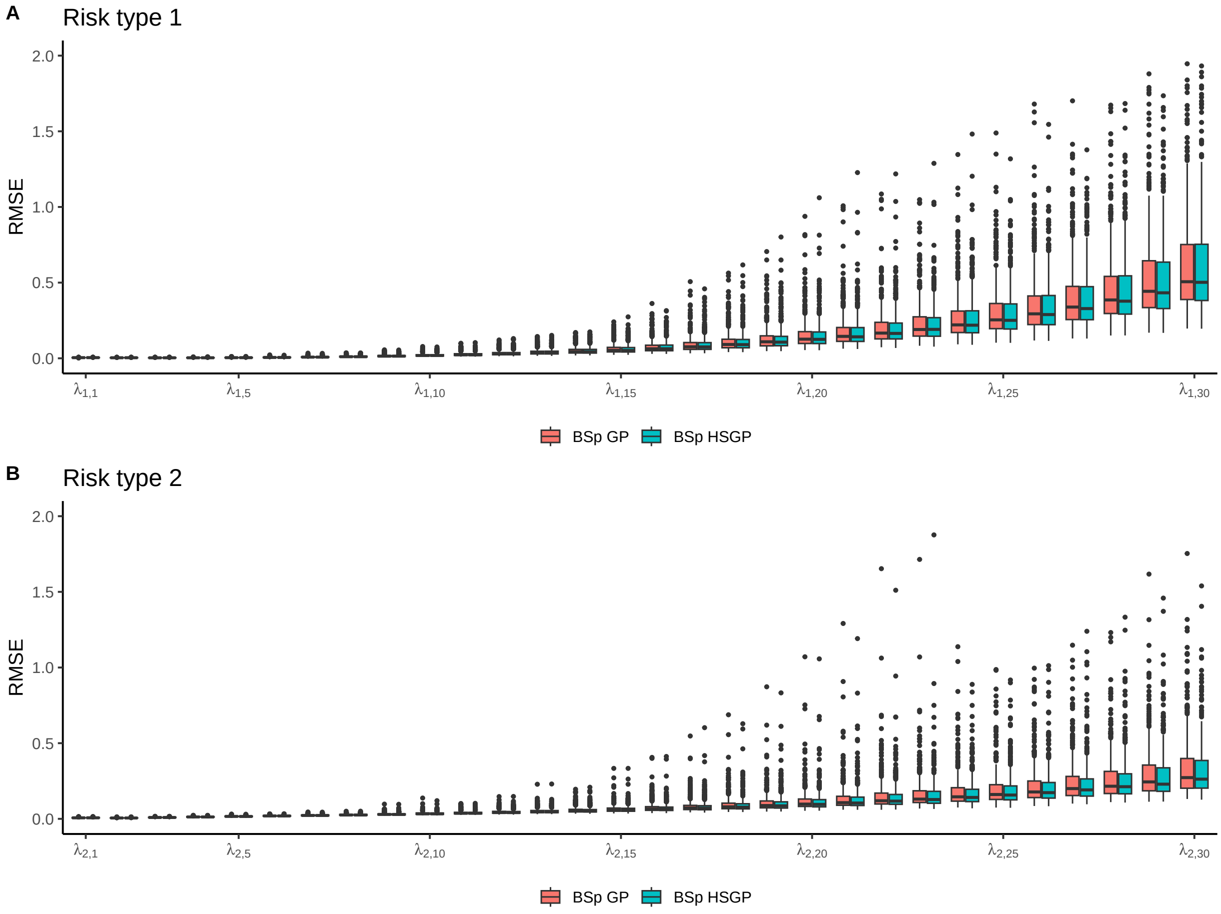


Figure 1: Simulation study, baseline hazard rates RMSE.

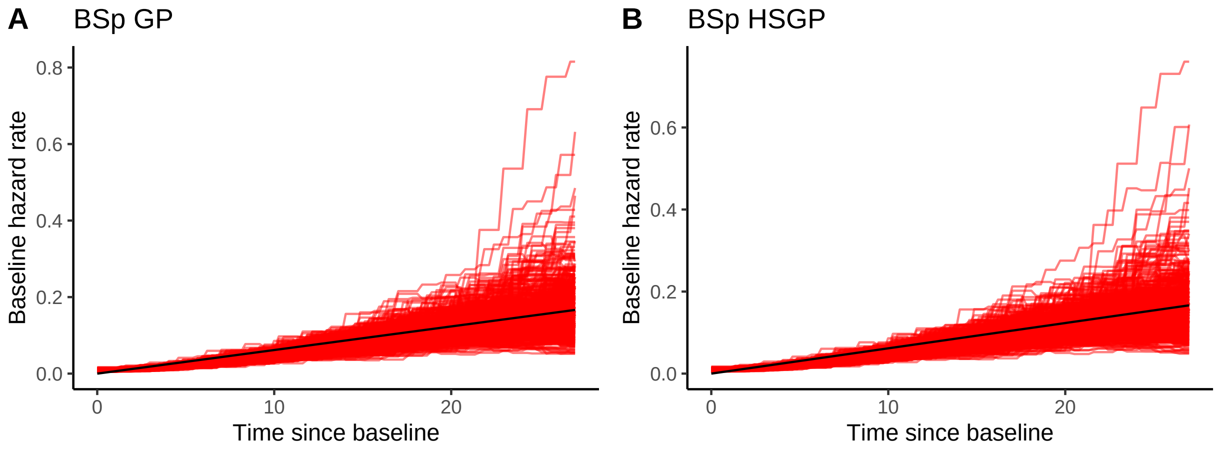


Figure 2: Risk type 2 baseline hazard rate results from simulation study with true hazard curves in black, and model fitted posterior means in red. Panel A: GP. Panel B: HSGP.

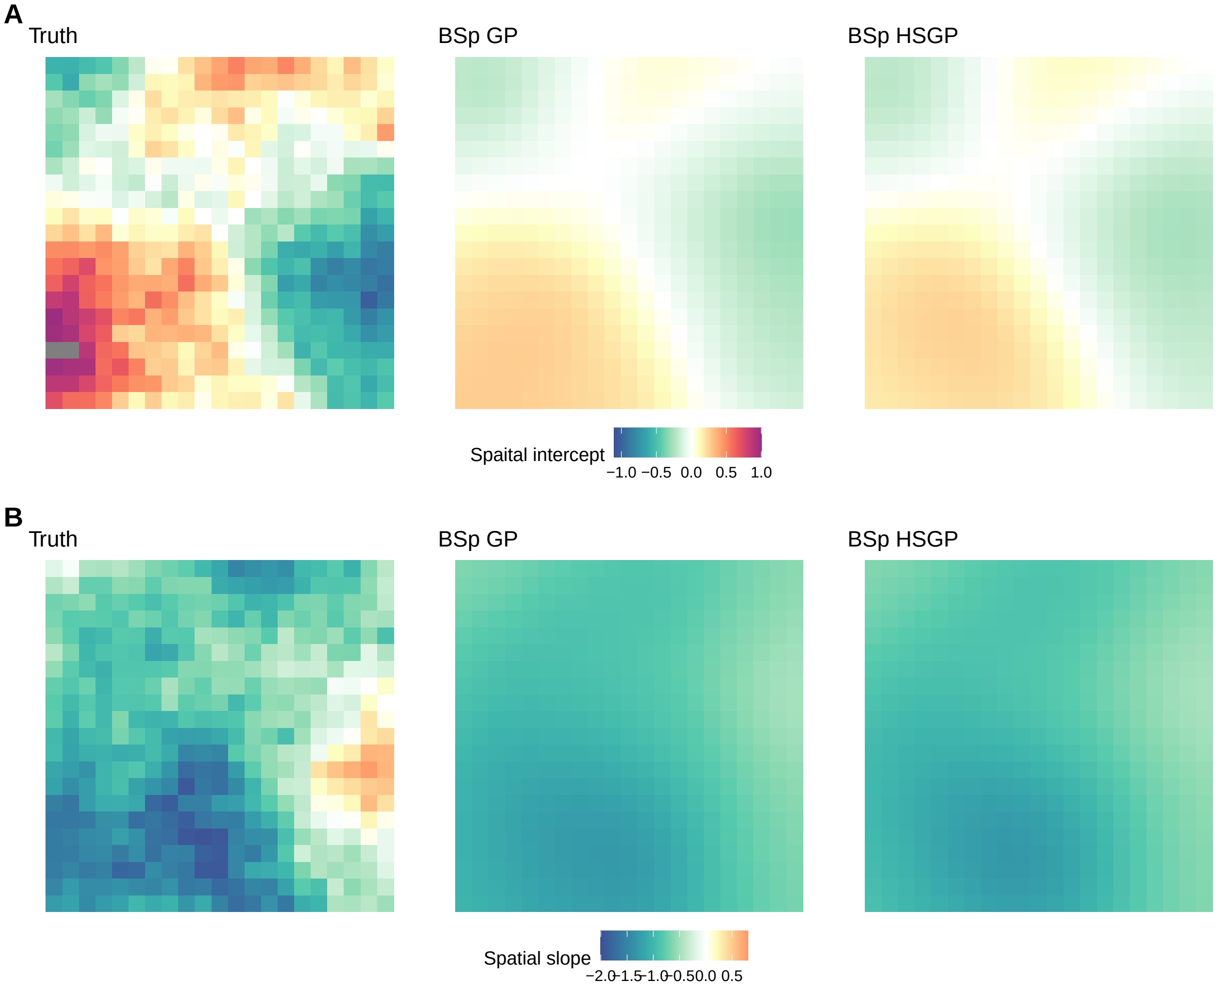


Figure 3: Risk type 2 spatial surface estimation results from simulation study. Panel A: the true spatial intercept surface, average of posterior means from GP and HSGP. Panel B: the true spatial slope surface, average of posterior means from GP and HSGP.

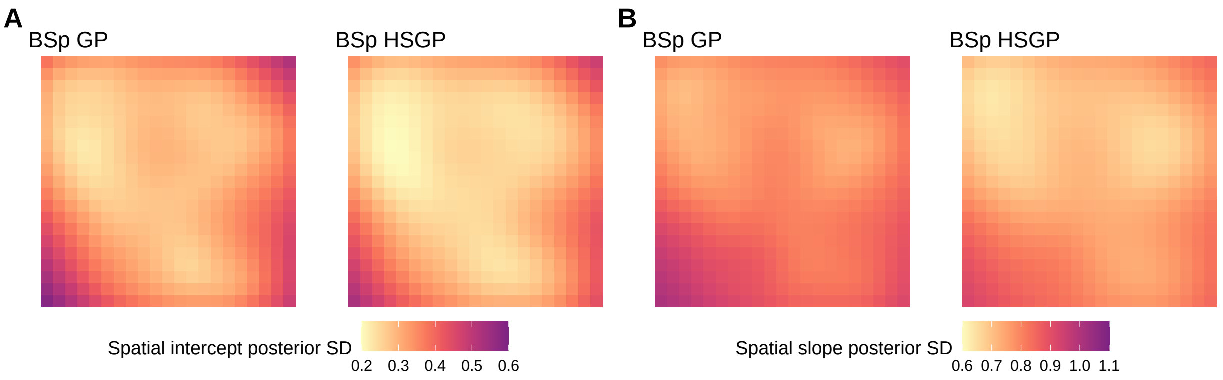


Figure 4: Average of posterior standard deviations for risk type 2 spatial surfaces from simulation study. Panel A: Spatial intercept results form GP and HSGP. Panel B: Spatial slope results from GP and HSGP.

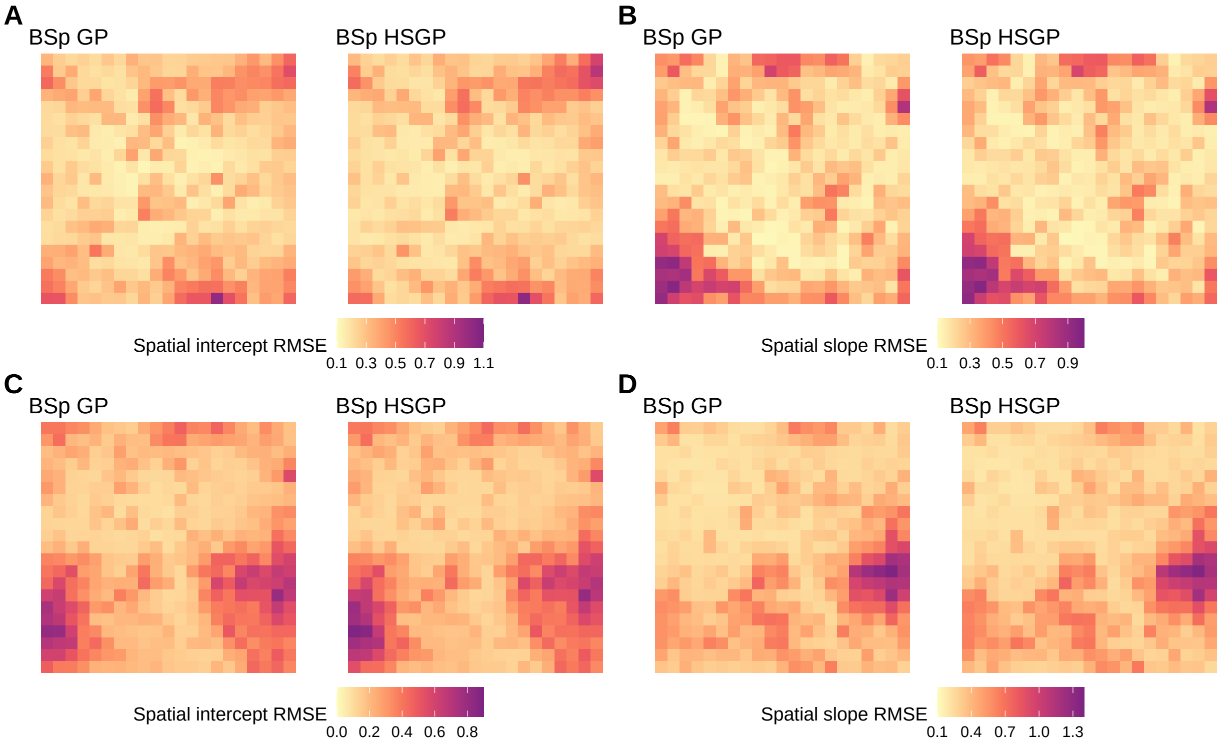


Figure 5: Average of RMSEs for spatial surfaces from simulation study. Panel A: Risk type 1 spatial intercept results. Panel B: Risk type 1 spatial slope results. Panel C: Risk type 2 spatial intercept results. Panel D: Risk type 2 spatial slope results.

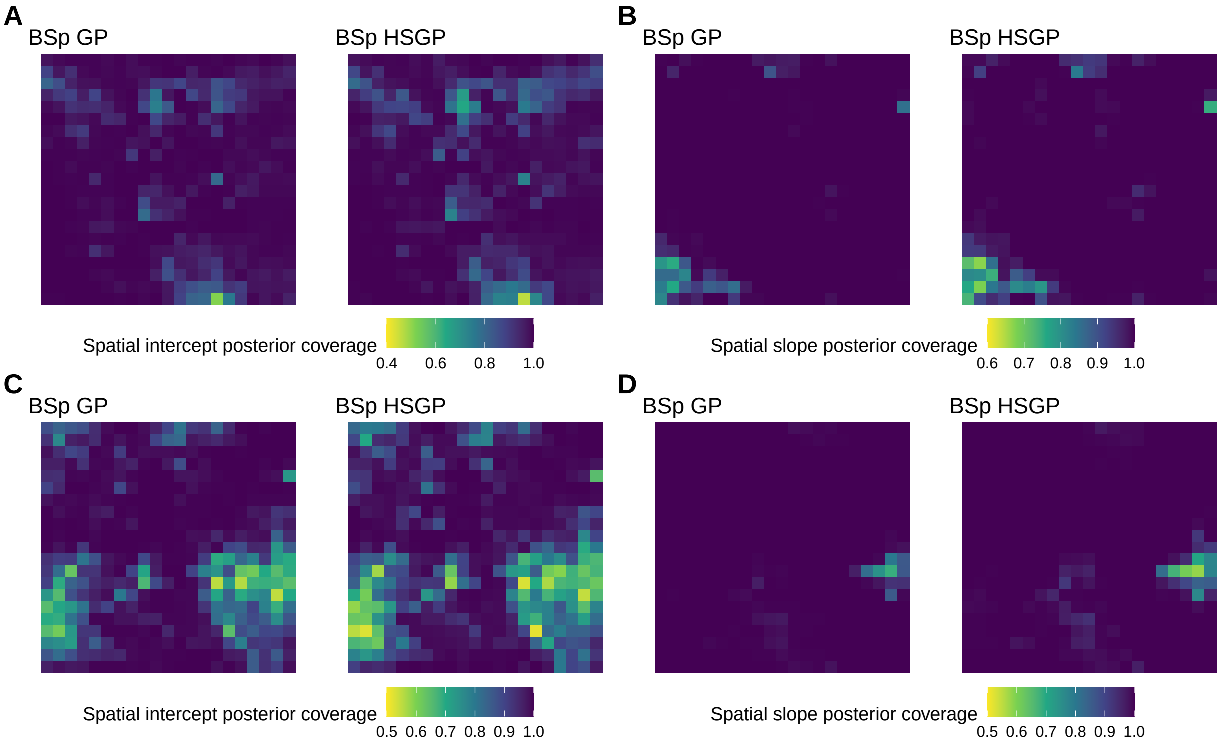


Figure 6: Posterior coverage results for spatial surfaces from simulation study. Panel A: Risk type 1 spatial intercept results. Panel B: Risk type 1 spatial slope results. Panel C: Risk type 2 spatial intercept results. Panel D: Risk type 2 spatial slope results.

# 6 Additional results for the application

In this section, we present additional results for the case study. Figure 7 shows traceplots for the regression coefficients for readmission risk. Figure 8 shows mortality risk spatial surface results.

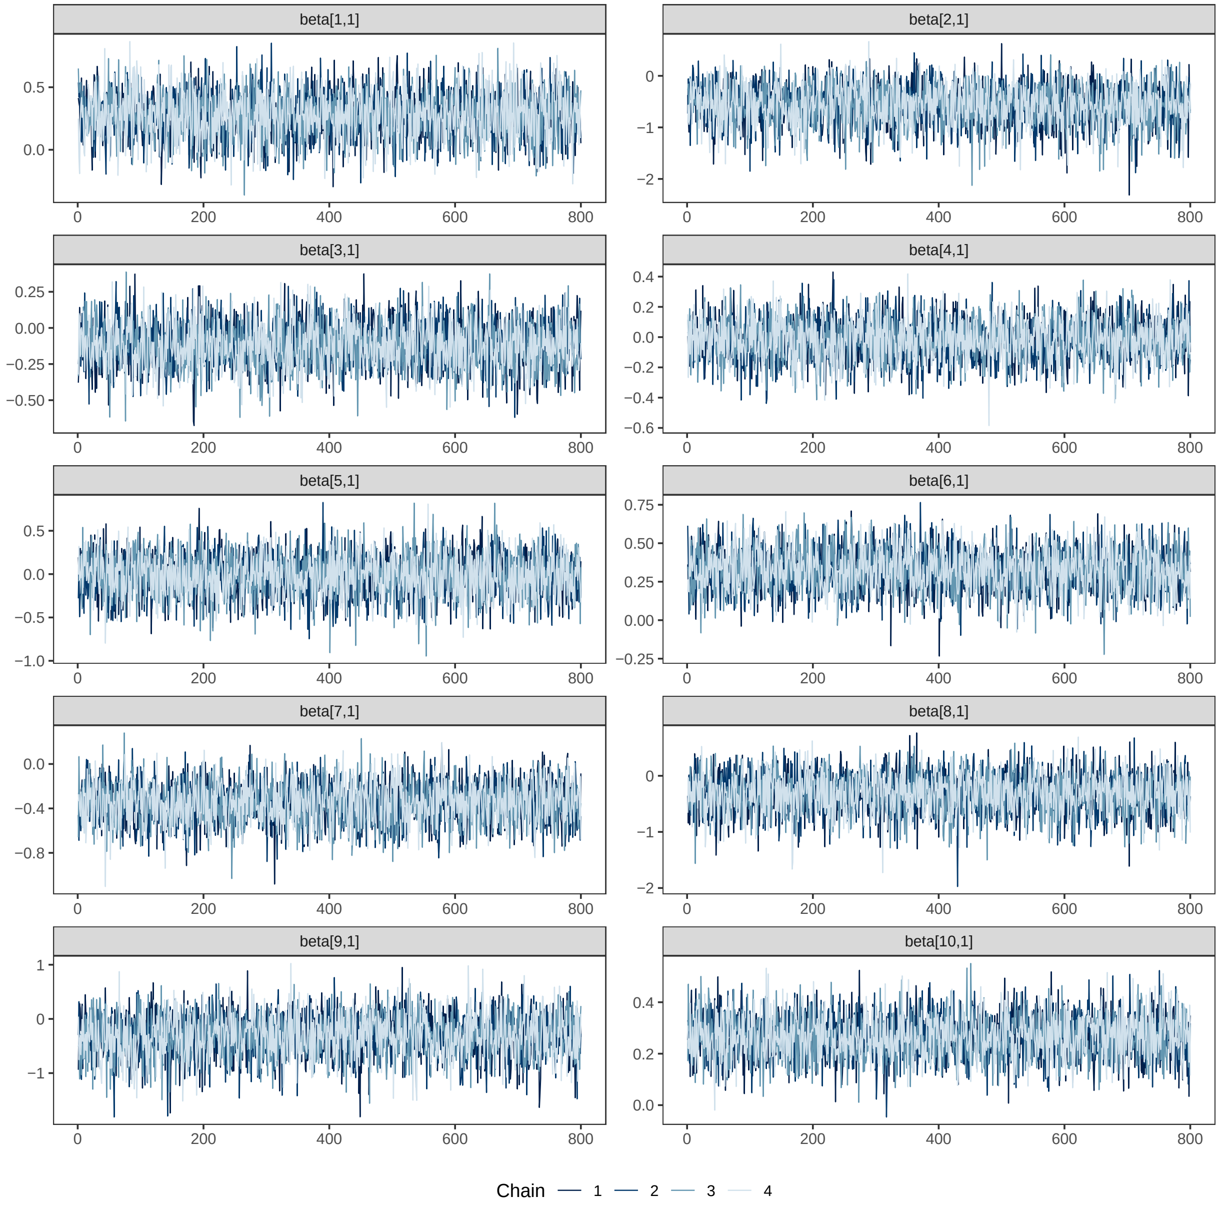


Figure 7: Traceplots for readmission risk regression coefficients, with $\beta[10, 1]$ as the fixed effects for comorbidity (denoted as $\beta_{w,1}$ in the article).

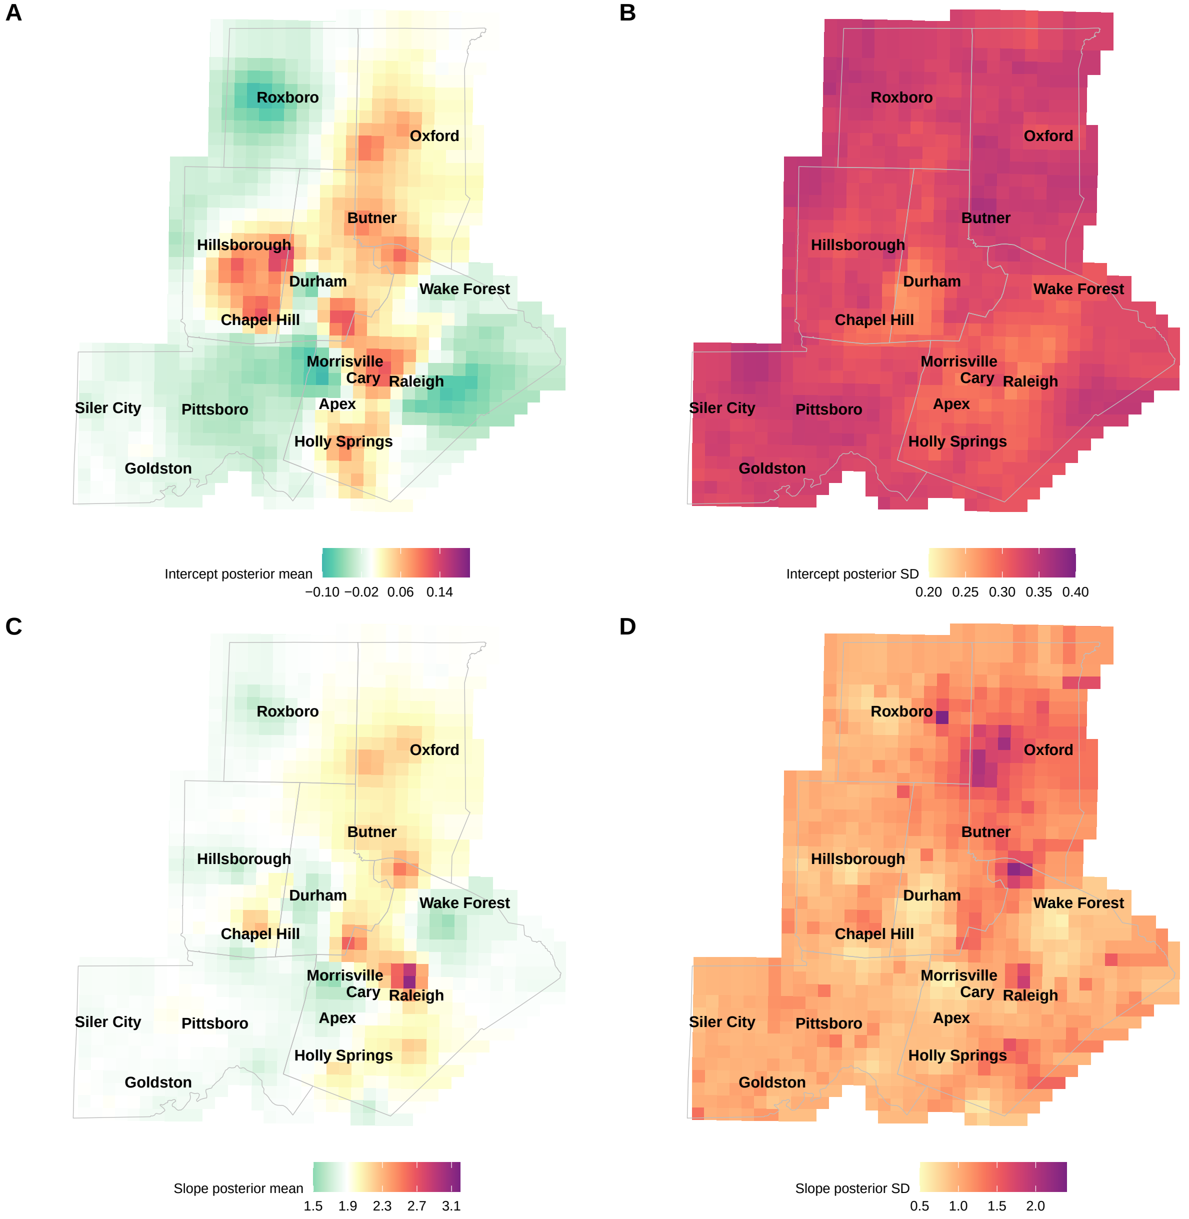


Figure 8: Posterior mean and standard deviation for mortality risk spatial surfaces. Panel A: Spatial intercept posterior mean. Panel B: Spatial intercept posterior standard deviation. Panel C: Spatial slope posterior mean. Panel D: Spatial slope posterior standard deviation.

# 7 Sensitivity Analysis

In this section we present results for the three sets of sensitivity tests on hyperparameters for the baseline hazard rates. Table 3 presents model comparison results, and the model with both spatial intercepts and slopes are consistently selected. Table 4 reports posterior mean and 95% posterior credible intervals for the readmission risk regression coefficients of the selected models.

Table 3: WAIC scores for sensitivity tests.

| Model | Low correlations | High correlations | $k = 100$ |
|---|---|---|---|
| BSp i+s | 4581.61 | 4569.90 | 4565.85 |
| BSp i | 4585.27 | 4574.37 | 4568.90 |
| BNSp | 4593.83 | 4582.30 | 4576.46 |

Table 4: Posterior means and 95% credible intervals for readmission risk regression coefficients (hazard ratio scale).

| | Low correlations | | High correlations | | $k = 100$ | |
|---|---|---|---|---|---|---|
| Variable | Mean | 95% CI | Mean | 95% CI | Mean | 95% CI |
| Age (per 1 SD) | 1.31 | (1.10, 1.54) | 1.31 | (1.11, 1.54) | 1.31 | (1.10, 1.54) |
| Comorbidity (per 1 SD) | 1.86 | (1.50, 2.31) | 1.91 | (1.52, 2.39) | 1.86 | (1.51, 2.33) |
| Female sex (baseline: Male) | 0.90 | (0.66, 1.21) | 0.90 | (0.66, 1.21) | 0.90 | (0.67, 1.2) |
| Race (baseline: White) | | | | | | |
| Black | 1.34 | (0.90, 1.89) | 1.35 | (0.92, 1.90) | 1.35 | (0.92, 1.90) |
| Other | 0.61 | (0.26, 1.14) | 0.61 | (0.26, 1.12) | 0.62 | (0.25, 1.16) |
| Single (baseline: With partner) | 1.40 | (1.07, 1.81) | 1.40 | (1.05, 1.81) | 1.39 | (1.05, 1.81) |
| Smoking status (baseline: Never) | | | | | | |
| Former | 0.99 | (0.76, 1.28) | 0.99 | (0.75, 1.27) | 0.99 | (0.75, 1.29) |
| Current | 1.01 | (0.61, 1.53) | 1.01 | (0.63, 1.55) | 1.02 | (0.62, 1.55) |
| Insurance (baseline: Government) | | | | | | |
| Commercial | 0.72 | (0.50, 0.99) | 0.71 | (0.48, 1.01) | 0.72 | (0.49, 1.00) |
| WCSC | 0.77 | (0.36, 1.36) | 0.77 | (0.36, 1.36) | 0.78 | (0.36, 1.41) |
| Selfpay | 0.79 | (0.32, 1.52) | 0.79 | (0.33, 1.53) | 0.79 | (0.33, 1.55) |

Figures 9-11 are posterior baseline hazard rate results for the sensitivity tests. There are more fluctuations in Figure 9 because of lower prior correlations between the piecewise-constant rates. Figure 10 has less fluctuations because of higher prior correlations. Figure

11 is denser because $k$ is set to 100, but it exhibits similar patterns as the base run results.

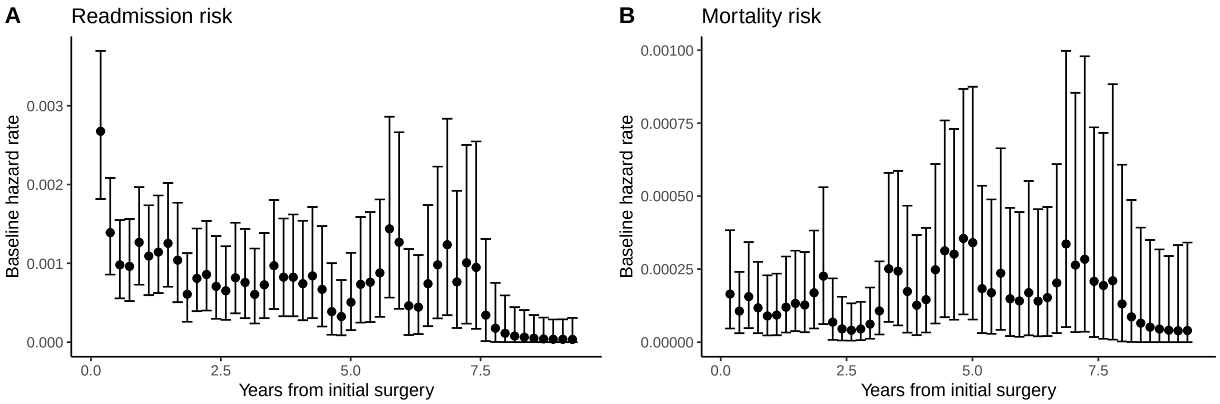


Figure 9: Posterior mean and 95% credible interval for the baseline hazard rates for low correlation sensitivity test. Panel A: Readmission risk. Panel B: Mortality risk.

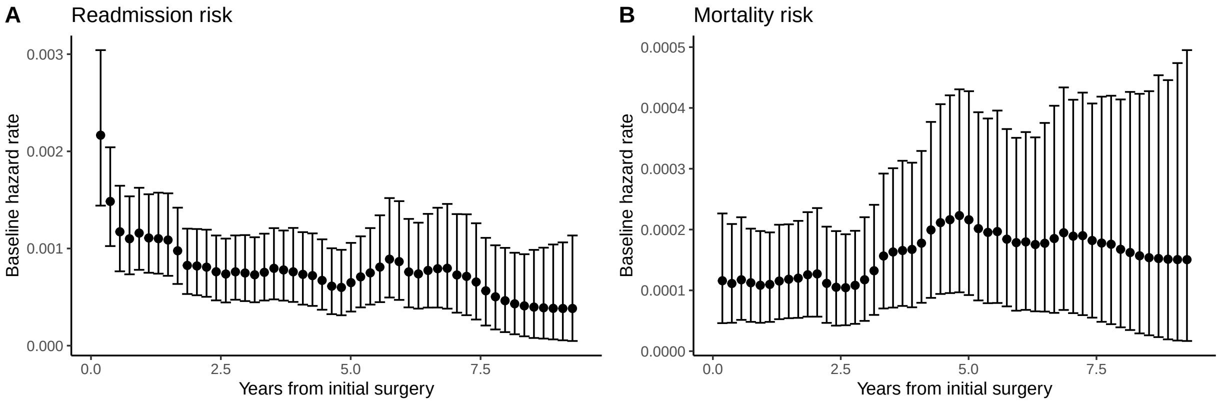


Figure 10: Posterior mean and 95% credible interval for the baseline hazard rates for high correlation sensitivity test. Panel A: Readmission risk. Panel B: Mortality risk.

Figures 12-14 present readmission risk spatial surface results, and Figures 15-17 are the clustering results. These results are similar to the base run.

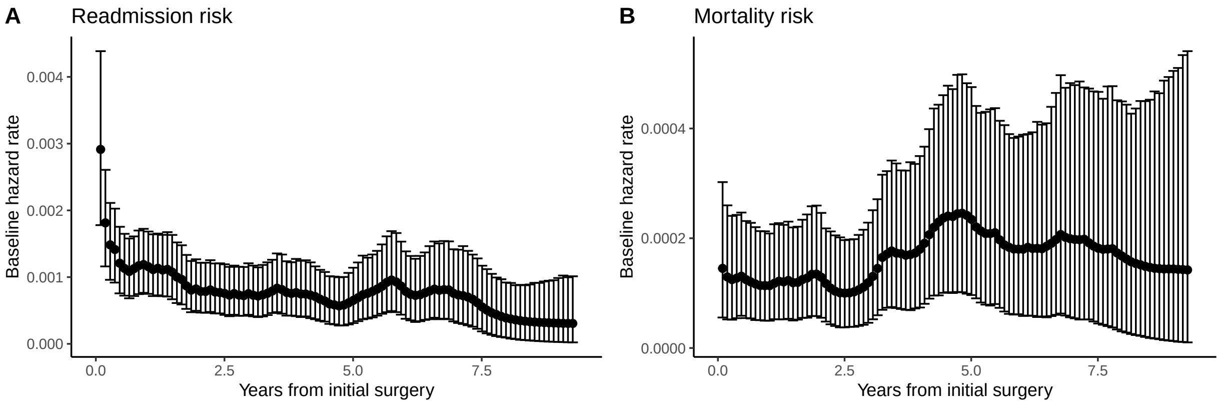


Figure 11: Posterior mean and 95% credible interval for the baseline hazard rates for $k = 100$ sensitivity test. Panel A: Readmission risk. Panel B: Mortality risk.

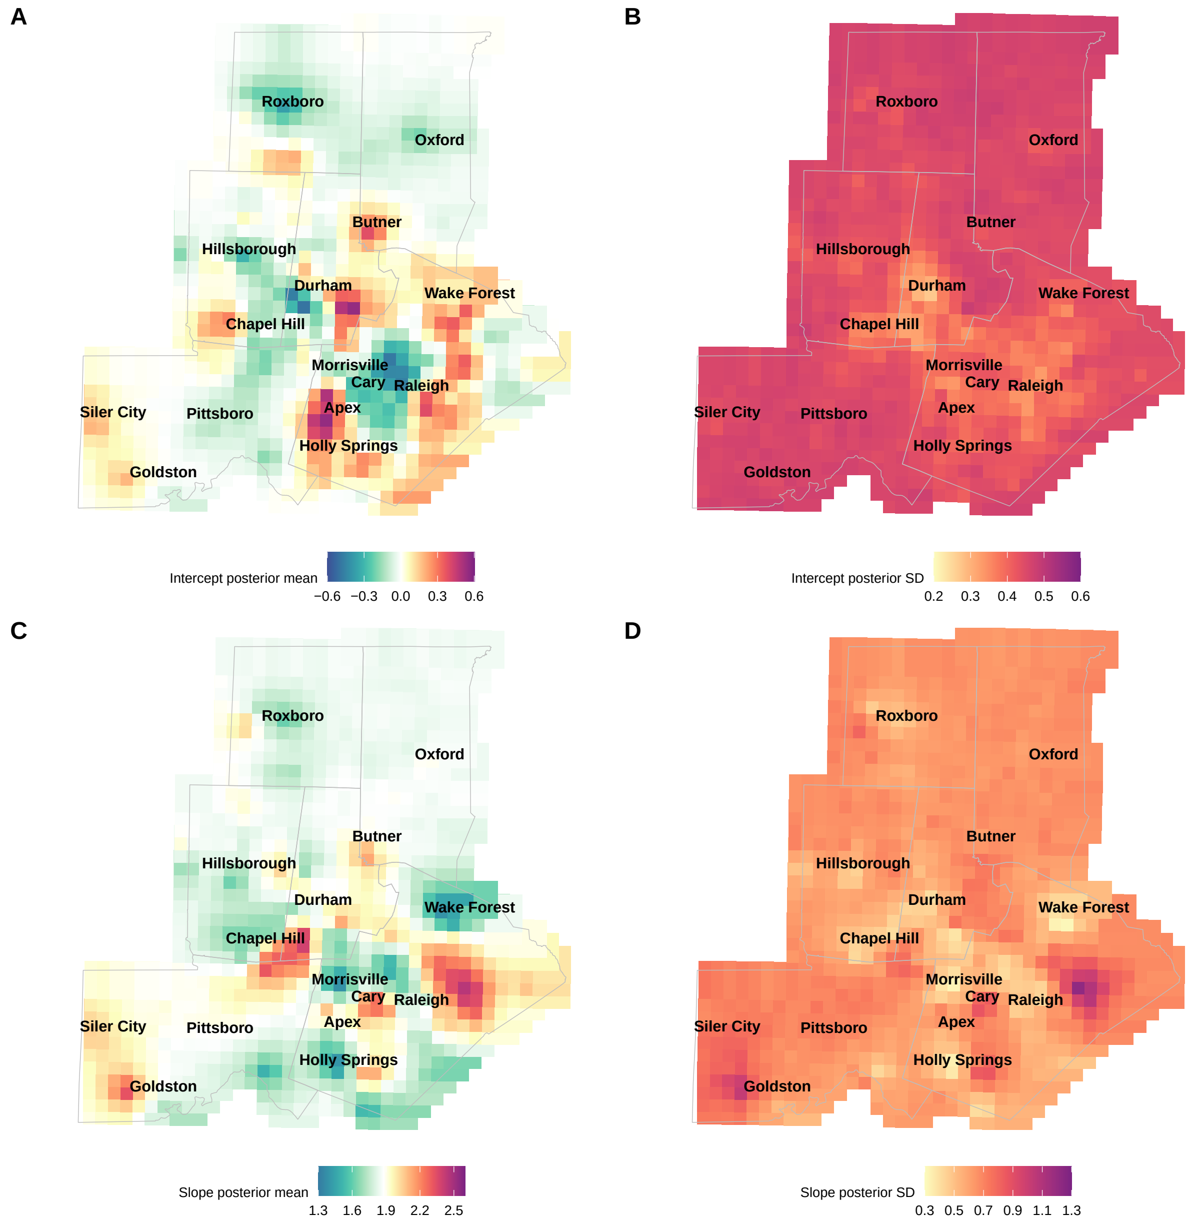


Figure 12: Posterior mean and standard deviation for readmission risk spatial surfaces for low correlation sensitivity test. Panel A: Spatial intercept posterior mean. Panel B: Spatial intercept posterior standard deviation. Panel C: Spatial slope posterior mean. Panel D: Spatial slope posterior standard deviation.

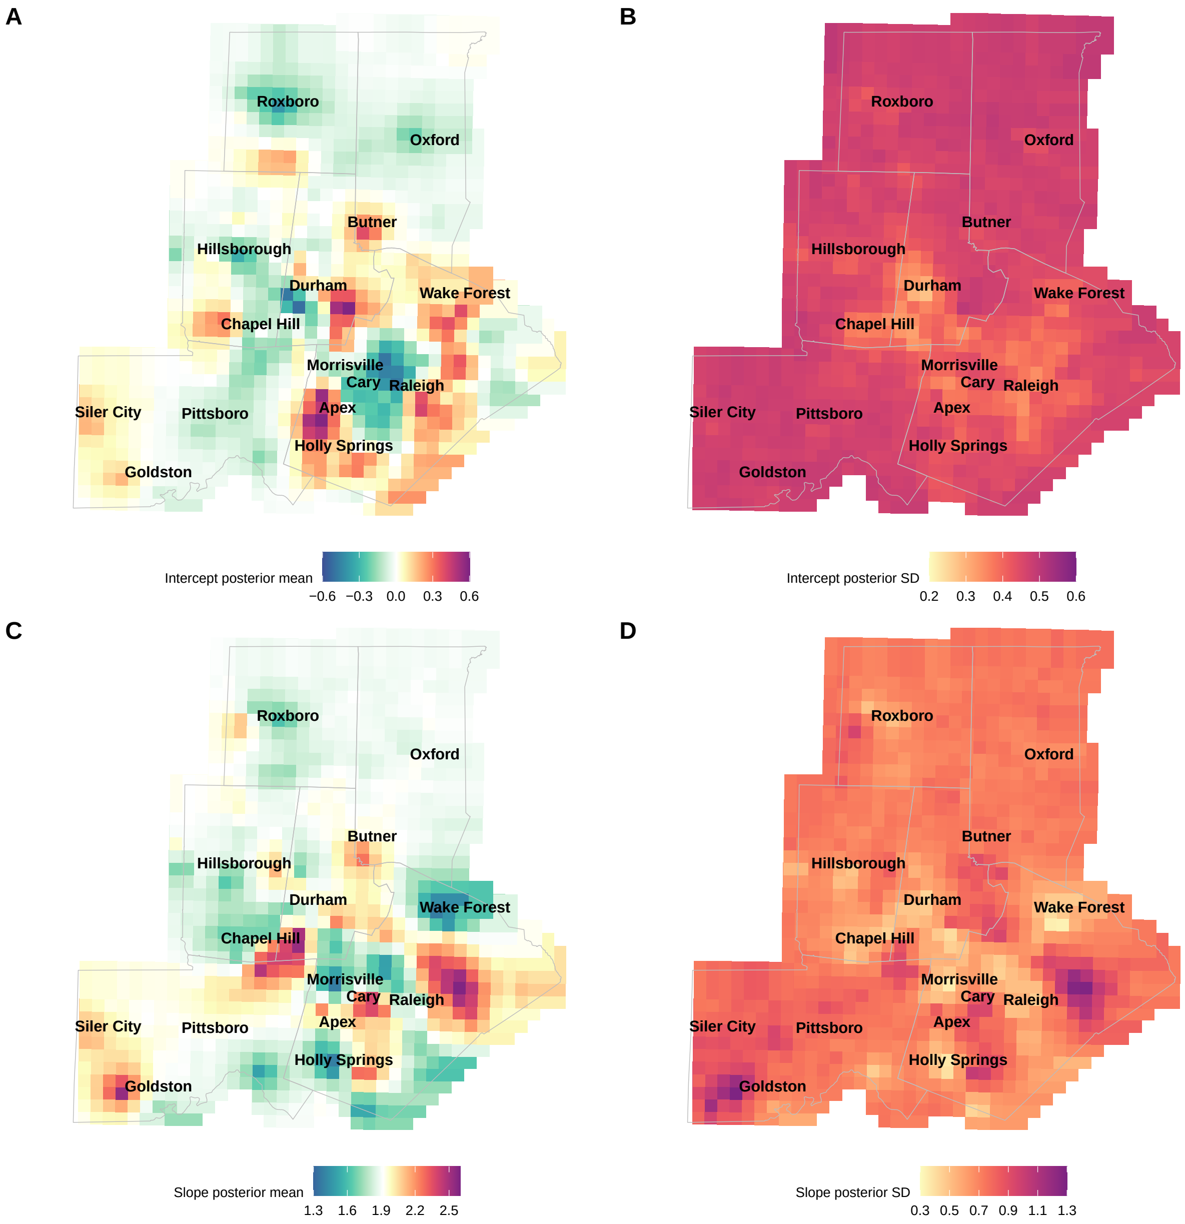


Figure 13: Posterior mean and standard deviation for readmission risk spatial surfaces for high correlation sensitivity test. Panel A: Spatial intercept posterior mean. Panel B: Spatial intercept posterior standard deviation. Panel C: Spatial slope posterior mean. Panel D: Spatial slope posterior standard deviation.

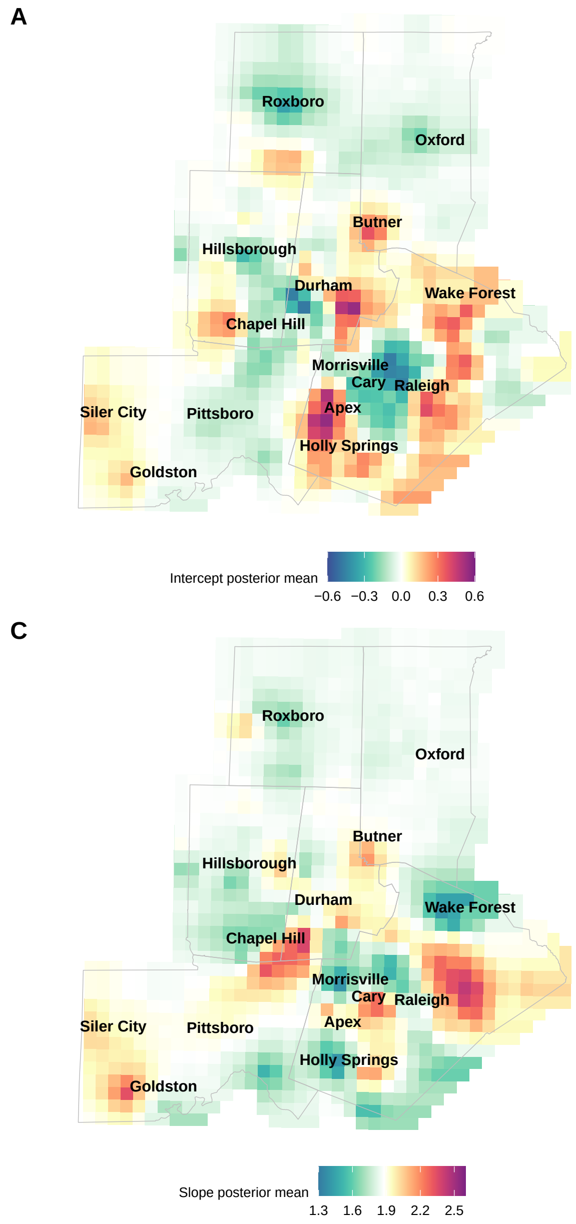


Figure 14: Posterior mean and standard deviation for readmission risk spatial surfaces for $k = 100$ sensitivity test. Panel A: Spatial intercept posterior mean. Panel B: Spatial intercept posterior standard deviation. Panel C: Spatial slope posterior mean. Panel D: Spatial slope posterior standard deviation.

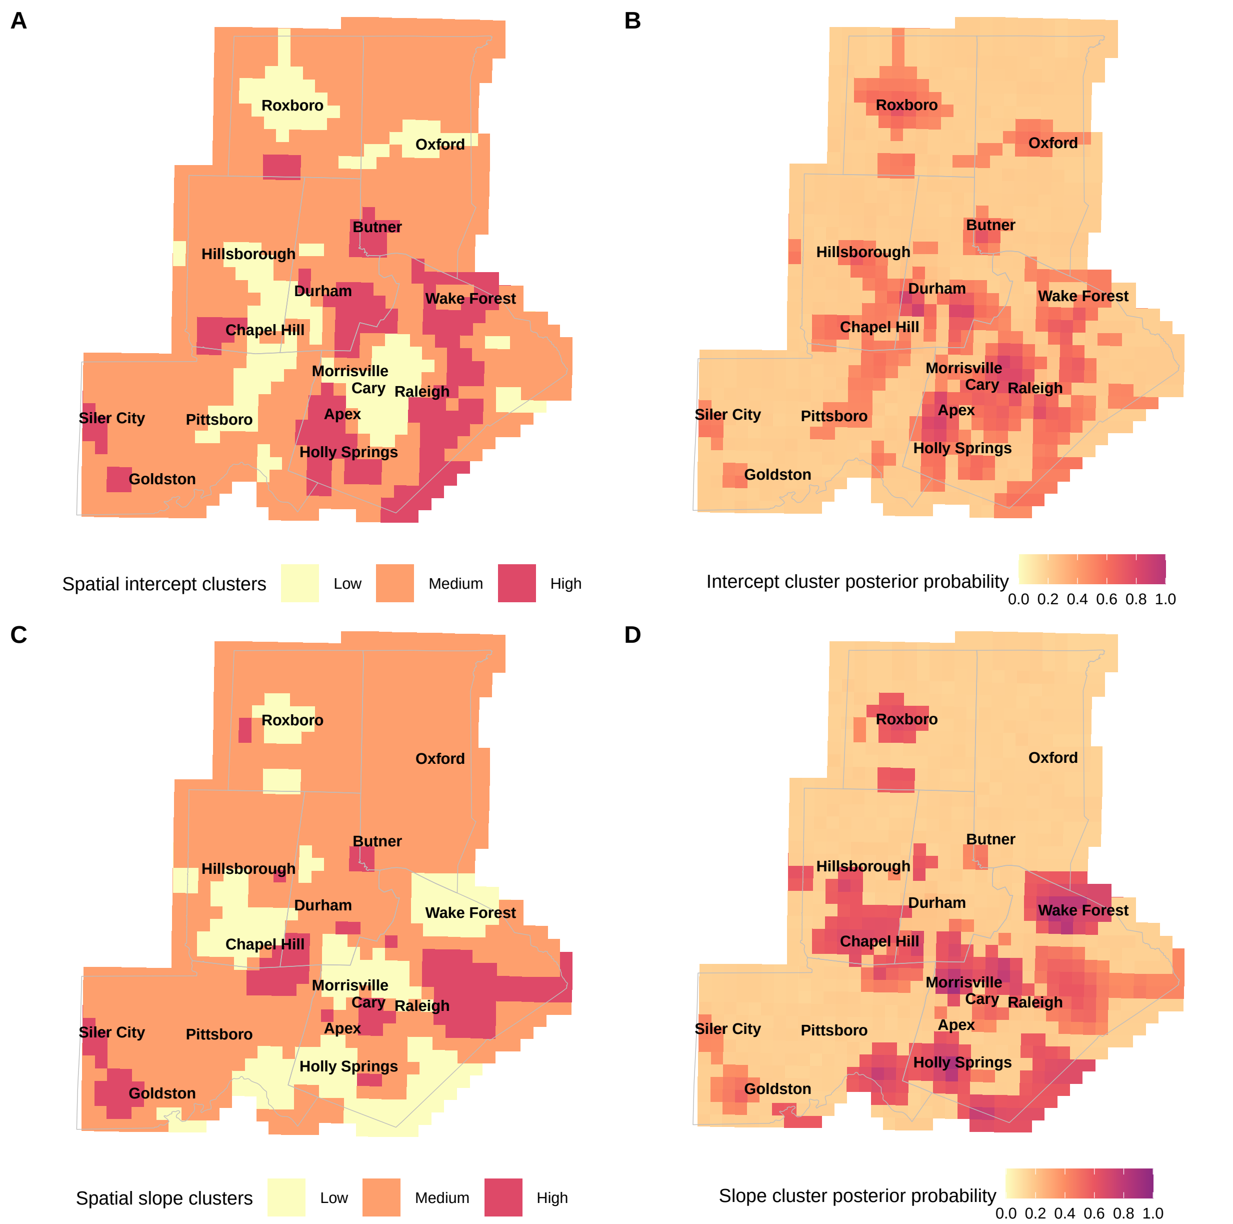


Figure 15: Clustering results for readmission risk spatial surfaces for low correlation sensitivity test. Panel A: Spatial intercept clusters with cluster means: -0.17, 0.00, and 0.20. Panel C: Spatial slope clusters with cluster means on hazard ratio scale: 1.69, 1.87, and 2.13. Panel B and D: Posterior probability of being in the estimated intercept / slope cluster.

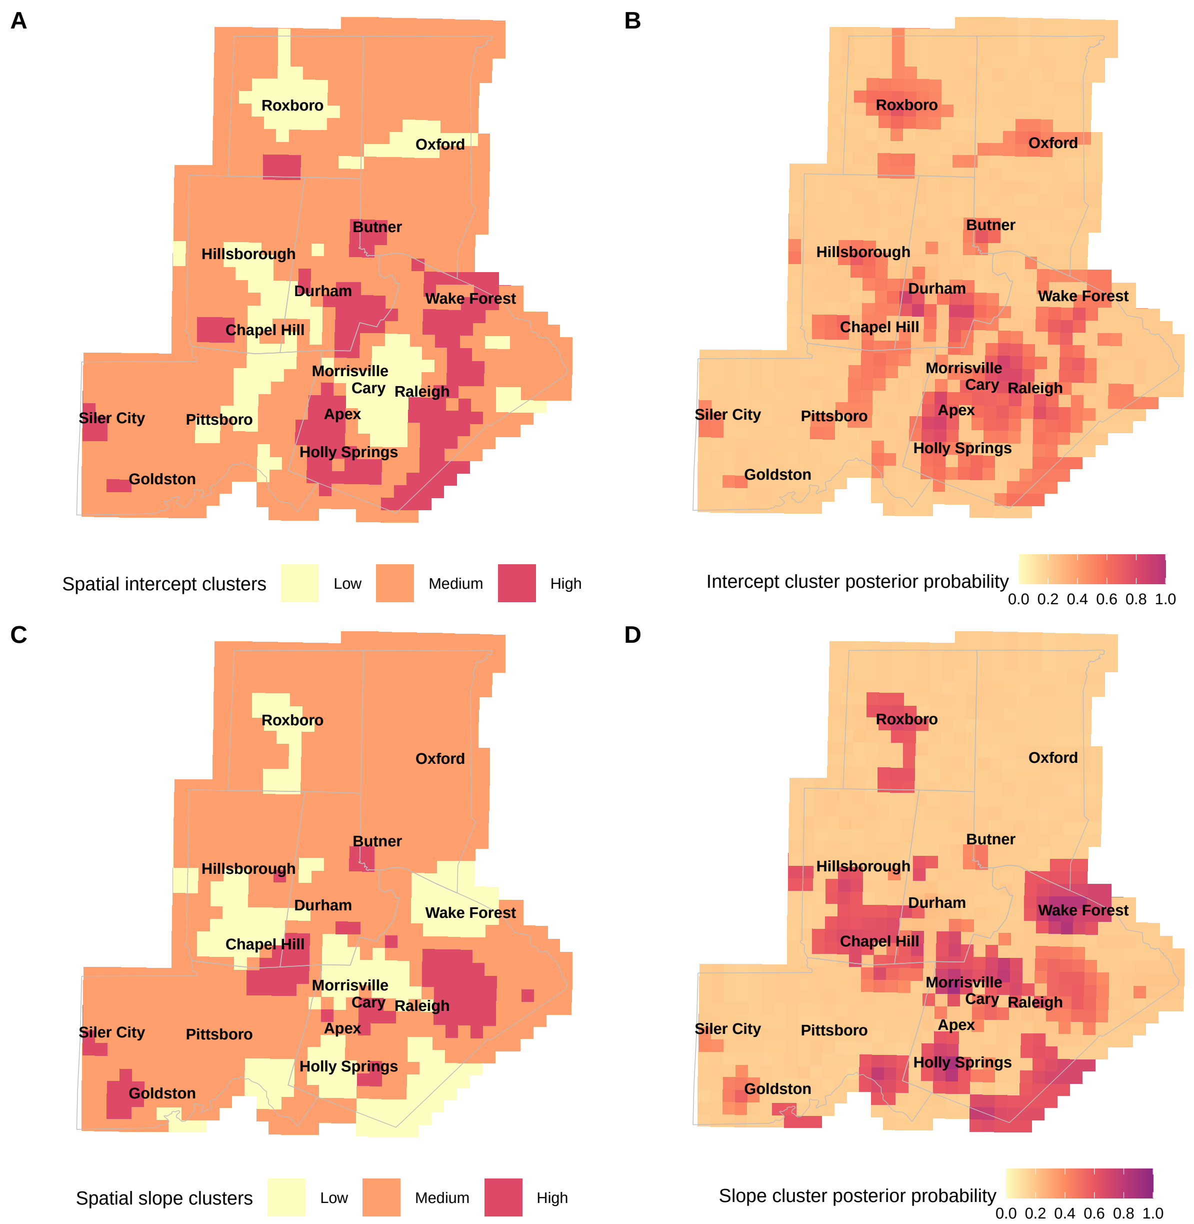


Figure 16: Clustering results for readmission risk spatial surfaces for high correlation sensitivity test. Panel A: Spatial intercept clusters with cluster means: -0.18, 0.00, and 0.23. Panel C: Spatial slope clusters with cluster means on hazard ratio scale: 1.71, 1.92, and 2.22. Panel B and D: Posterior probability of being in the estimated intercept / slope cluster.

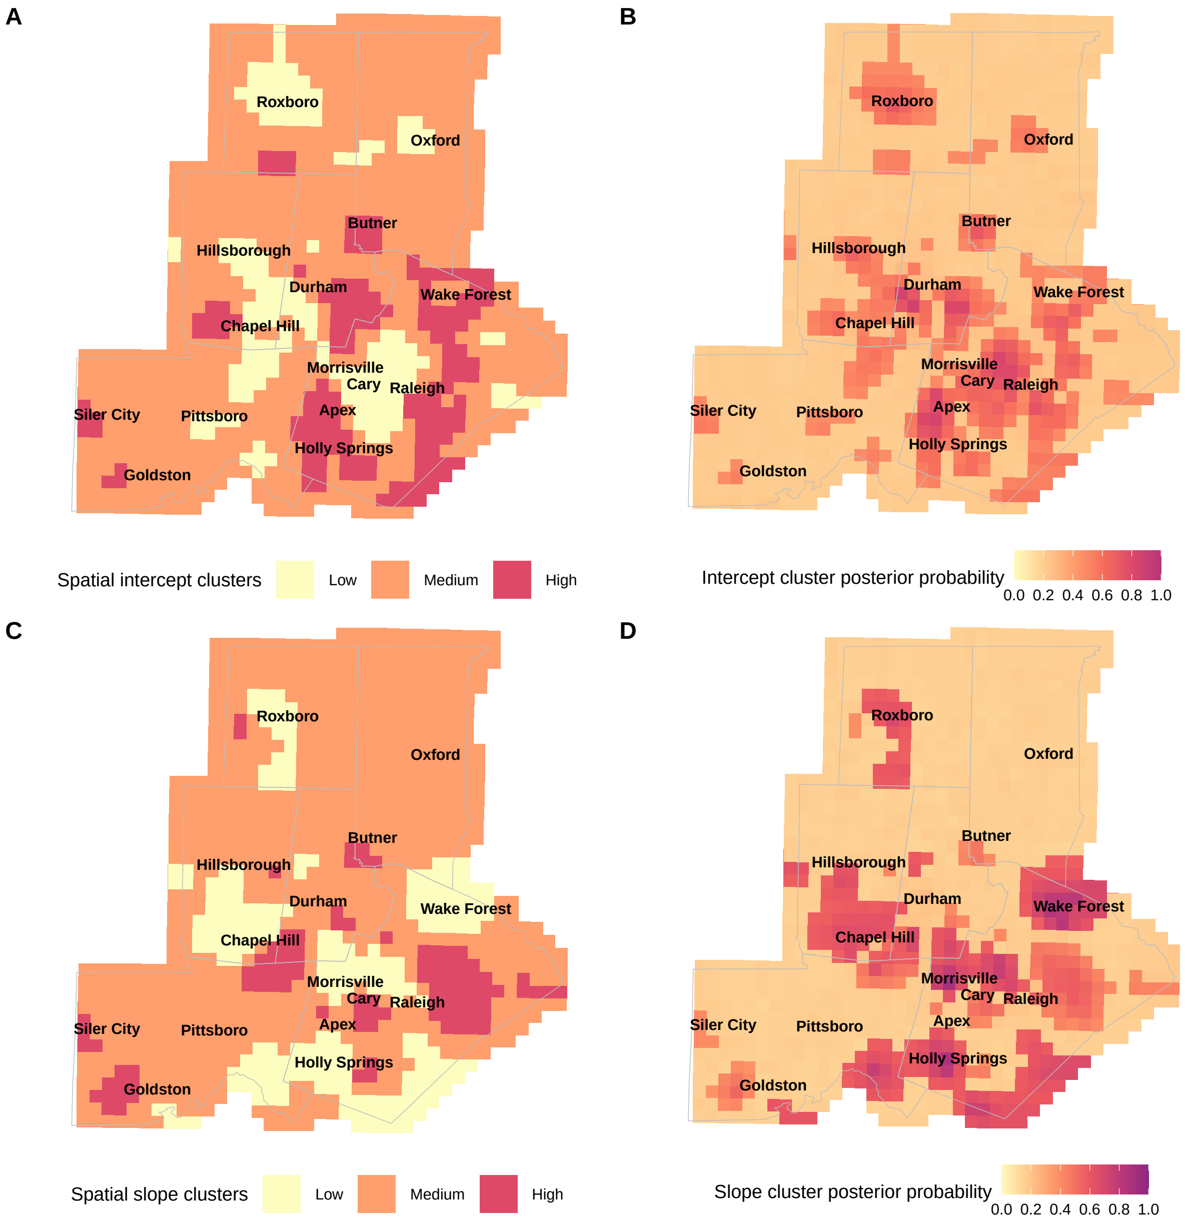


Figure 17: Clustering results for readmission risk spatial surfaces for $k = 100$ sensitivity test. Panel A: Spatial intercept clusters with cluster means: -0.18, 0.00, and 0.21. Panel C: Spatial slope clusters with cluster means on hazard ratio scale: 1.69, 1.87, and 2.14. Panel B and D: Posterior probability of being in the estimated intercept / slope cluster.
